# Supplementary material for: Local SGD Optimizes Overparameterized Neural Networks in Polynomial Time
Source: arXiv:2107.10868 source file (2022-02-22)
Supplement: Supplementary file 1 [file appendix.tex]

\clearpage
 \appendix

\section{Proof of Theorem~\ref{theorem: local GD}  (Local GD)}\label{app: GD}
In this section  we are going to present the proof of convergence rate of Local GD (Theorem~\ref{theorem: local GD}). Before that, let us first introduce some useful lemmas. 
\subsection{Proof of Technical Lemma}
The following lemma is from Allen-Zhu et al's seminal work~\cite{allen2019convergence}, which characterizes the bounded number of changed pattern after ReLU activation:
\begin{lemma}[Allen et al~\cite{allen2019convergence}]\label{lemma:perturbation}
Consider a weight matrices $\tilde{\mathbf{W}} $, $\mathbf{W}$ such that $\tilde{\mathbf{W}}, \mathbf{W}\in\mathcal{B}(\mathbf{W}(0),\omega)$, with probability at least $1-\exp(-O(m\omega^{2/3}))$, there exists constants $C'$, $C''$  such that
\begin{align*} 
     \|\tilde{\mathbf{D}}_{ i} -  \mathbf{D}_{ i}\big\|_0\le C'\omega^{2/3},  \|(\tilde{\mathbf{D}}_{ i} - \mathbf{D}_{ i})\bm{v}\|_2\le C''\omega^{1/3} \sqrt{m\log(m)}/\sqrt{d},  
\end{align*} 
where $\tilde{\mathbf{D}}_{i}$ and ${\mathbf{D}}_{i}$ are $m\times m$-dimensional diagonal matrix with entries $\tilde{\mathbf{D}}_{i}(r,r) = \sigma'(\langle \tilde{\mathbf{W}}_r, \bm{x}_i \rangle)$ and $ {\mathbf{D}}_{i}(r,r) = \sigma'(\langle \mathbf{W}_r, \bm{x}_i \rangle)$.
\end{lemma}

\begin{lemma}
\begin{align*}
 \left\| \mathbf{W}^{(i)}(t) -  \mathbf{W}(t_c) \right\|^2_{\mathrm{F}}  
    & \leq     O\left((\eta^2 \tau^2   + \eta^2 \tau)\frac{mn}{d}\right) L_i(\mathbf{W}(t_c) ). 
\end{align*}
\begin{proof}
According to updating rule:
\begin{align*}
    \left\| \mathbf{W}^{(i)}(t+1) -  \mathbf{W}(t_c) \right\|^2_{\mathrm{F}} =   &\left\| \mathbf{W}^{(i)}(t) - \eta \nabla L_i(\mathbf{W}^{(i)}(t))- \mathbf{W}(t_c) \right\|^2_{\mathrm{F}}  \\
    & = \left\| \mathbf{W}^{(i)}(t) - \mathbf{W}(t_c) \right\|^2_{\mathrm{F}} - 2\eta \left \langle \nabla L_i(\mathbf{W}^{(i)}(t)), \mathbf{W}^{(i)}(t) - \mathbf{W}(t_c) \right\rangle\\
    &\quad  + \eta^2 \|\nabla L_i(\mathbf{W}^{(i)}(t))\|^2_\mathrm{F}\\
    & = \left\| \mathbf{W}^{(i)}(t) - \mathbf{W}(t_c) \right\|^2_{\mathrm{F}} + 2\eta \left \langle \nabla L_i(\mathbf{W}^{(i)}(t)),  \eta \sum_{t' = t_c}^{t-1} \nabla L_i(\mathbf{W}^{(i)}(t)) \right\rangle\\
    &\quad  + \eta^2 \|\nabla L_i(\mathbf{W}^{(i)}(t))\|^2_\mathrm{F}\\
     & = \left\| \mathbf{W}^{(i)}(t) - \mathbf{W}(t_c) \right\|^2_{\mathrm{F}} + 2\eta^2 \tau \left \langle \nabla L_i(\mathbf{W}^{(i)}(t)),   \frac{1}{\tau} \sum_{t' = t_c}^{t-1} \nabla L_i(\mathbf{W}^{(i)}(t)) \right\rangle\\
    &\quad  + \eta^2 \|\nabla L_i(\mathbf{W}^{(i)}(t))\|^2_\mathrm{F} 
\end{align*}
Applying the identity $\langle \bm{a}, \bm{b} \rangle = \frac{1}{2}\|\bm{a}\|^2+\frac{1}{2}\|\bm{b}\|^2 - \frac{1}{2}\|\bm{a}-\bm{b}\|^2$ on the cross term we have:
 \begin{align*}
    \left\| \mathbf{W}^{(i)}(t+1) -  \mathbf{W}(t_c) \right\|^2_{\mathrm{F}} =   &\left\| \mathbf{W}^{(i)}(t) - \eta \nabla L_i(\mathbf{W}^{(i)}(t))- \mathbf{W}(t_c) \right\|^2_{\mathrm{F}}  \\
     & \leq \left\| \mathbf{W}^{(i)}(t) - \mathbf{W}(t_c) \right\|^2_{\mathrm{F}} +  \eta^2 \tau \left(\left \| \nabla L_i(\mathbf{W}^{(i)}(t))\right\|^2+\left \|   \frac{1}{\tau} \sum_{t' = t_c}^{t-1} \nabla L_i(\mathbf{W}^{(i)}(t)) \right\|^2 \right)\\
    &\quad  + \eta^2 \|\nabla L_i(\mathbf{W}^{(i)}(t))\|^2_\mathrm{F} \\
    & \leq \left\| \mathbf{W}^{(i)}(t) - \mathbf{W}(t_c) \right\|^2_{\mathrm{F}} +  \eta^2 (t-t_c) \left(\left \| \nabla L_i(\mathbf{W}^{(i)}(t))\right\|^2+ \frac{1}{t-t_c} \sum_{t' = t_c}^{t-1}\left \|   \nabla L_i(\mathbf{W}^{(i)}(t)) \right\|^2 \right)\\
    &\quad  + \eta^2 \|\nabla L_i(\mathbf{W}^{(i)}(t))\|^2_\mathrm{F} \\
\end{align*}
Plugging the gradient upper bound from Lemma~\ref{lemma:grad bounds} yields:
 \begin{align*}
    \left\| \mathbf{W}^{(i)}(t+1) -  \mathbf{W}(t_c) \right\|^2_{\mathrm{F}} =   &\left\| \mathbf{W}^{(i)}(t) - \eta \nabla L_i(\mathbf{W}^{(i)}(t))- \mathbf{W}(t_c) \right\|^2_{\mathrm{F}}  \\ 
    & \leq \left\| \mathbf{W}^{(i)}(t) - \mathbf{W}(t_c) \right\|^2_{\mathrm{F}} +  \eta^2 (t-t_c) \left(O\big(\frac{mn}{d}\big) L_i(\mathbf{W}^{(i)}(t) ) + \frac{1}{t-t_c} \sum_{t' = t_c}^{t-1}O\big(\frac{mn}{d}\big) L_i(\mathbf{W}^{(i)}(t') )  \right)\\
    &\quad  + \eta^2 O\big(\frac{mn}{d}\big) L_i(\mathbf{W}^{(i)}(t) )  
\end{align*}
Since we assume $L_i(\mathbf{W}^{(i)}(t) ) \leq L_i(\mathbf{W}(t_c) )$ for any $t_c \leq t\leq t_c + \tau -1$, we have:
 \begin{align*}
    \left\| \mathbf{W}^{(i)}(t+1) -  \mathbf{W}(t_c) \right\|^2_{\mathrm{F}} =   &\left\| \mathbf{W}^{(i)}(t) - \eta \nabla L_i(\mathbf{W}^{(i)}(t))- \mathbf{W}(t_c) \right\|^2_{\mathrm{F}}  \\ 
    & \leq \left\| \mathbf{W}^{(i)}(t) - \mathbf{W}(t_c) \right\|^2_{\mathrm{F}} +  \eta^2 \tau \left(O\big(\frac{mn}{d}\big) L_i(\mathbf{W}^{(i)}(t_c) ) +  O\big(\frac{mn}{d}\big) L_i(\mathbf{W}^{(i)}(t_c) )  \right)\\
    &\quad  + \eta^2 O\big(\frac{mn}{d}\big) L_i(\mathbf{W}^{(i)}(t_c) )  
\end{align*}
Do the telescoping sum from $t+1$ to $t_c$ will conclude the proof:
 \begin{align*}
    \left\| \mathbf{W}^{(i)}(t+1) -  \mathbf{W}(t_c) \right\|^2_{\mathrm{F}}  
    & \leq     O\left((\eta^2 \tau^2   + \eta^2 \tau)\frac{mn}{d}\right) L_i(\mathbf{W}^{(i)}(t_c) ). 
\end{align*}

\end{proof}

\end{lemma}

The following lemma establishes a bound on the deviation between local models and (virtual) averaged global model in terms of global loss.
\begin{lemma}\label{lemma: weight gap GD}
For Local GD, let $t_c$ denote  the latest communication stage of before iteration $t$. Then the following statement holds true for $t_c \leq t \leq t_c + \tau$:
\begin{align*}
  \frac{1}{K}\sum_{i=1}^K \left\| \mathbf{W}^{(i)}(t) -  \mathbf{W}(t) \right\|^2_{\mathrm{F}} \leq \left(\frac{16m^3n^3 \tau^3 \eta^4}{d^3}+ \frac{4mn\tau \eta^2}{d}\right)\sum_{t'=t_c}^{t-1} L(\mathbf{W}(t')),
\end{align*}
where $K$ is the number of devices, $\tau$ is the number of local updates between two consecutive rounds of synchronization, $n$ is the size of each local data shard, and $m$ is the number of neurons in hidden layer.

\begin{proof}
According to updating rule of Local GD: 
\begin{align*}
 &\frac{1}{K}\sum_{i=1}^K \left\| \mathbf{W}^{(i)}(t) -  \mathbf{W}(t) \right\|^2_{\mathrm{F}} \nonumber\\
 & \leq  \eta^2 \frac{1}{K}\sum_{i=1}^K  \left\|  \sum_{t'=t_c}^{t-1}\left( \nabla L_i (\mathbf{W}^{(i)}(t') )   -   \frac{1}{K}\sum_{j=1}^K  \nabla  L_j (\mathbf{W}^{(j)}(t'))  \right)\right\|^2_{\mathrm{F}} \stackrel{\text{\ding{192}}}{\leq} (t-t_c)\eta^2 \frac{1}{K}\sum_{i=1}^K  \sum_{t'=t_c}^{t-1} \left\|   \nabla L_i (\mathbf{W}^{(i)}(t') )  \right\|^2_{\mathrm{F}}\\
  &= (t-t_c)\eta^2 \frac{1}{K}\sum_{i=1}^K  \sum_{t'=t_c}^{t-1} \sum_{r=1}^m\left\|  \frac{1}{\sqrt{d}}\sum_{(\bm{x},y)\in S_i} \left(f(\mathbf{W}^{(i)}(t),\bm{v},\bm{x}) - y \right) a_r \bm{x} \sigma'(\mathbf{W}_r^{(i)}(t')^\top \bm{x})   \right\|^2_{\mathrm{F}}\\ 
    &\stackrel{\text{\ding{193}}}{\leq} (t-t_c)m\eta^2 \frac{1}{ dK}\sum_{i=1}^K   \sum_{t'=t_c}^{t-1}  n \sum_{(\bm{x},y)\in S_i} \left(2 \left\|f(\mathbf{W}^{(i)}(t'),\bm{v},\bm{x}) - f(\mathbf{W}(t'),\bm{v},\bm{x})    \right\|^2_{\mathrm{F}} +2 \left\|f(\mathbf{W}(t'),\bm{v},\bm{x}) - y    \right\|^2_{\mathrm{F}}\right)\\ 
   &\leq(t-t_c)m\eta^2 \frac{1}{ dK}\sum_{i=1}^K \sum_{t'=t_c}^{t-1} n  \sum_{(\bm{x},y)\in S_i} \left(2\left\| \frac{1}{\sqrt{d}} \sum_{r'=1}^m a_{r'} \left[ \sigma(\mathbf{W}_{r'}^{(i)}(t')\bm{x}  ) - \sigma(\mathbf{W}_{r'}(t')\bm{x}  )\right]   \right\|^2_{\mathrm{F}}    + 2\left\|   f(\mathbf{W}(t'),\bm{v},\bm{x}) - y   \right\|^2_{\mathrm{F}}\right)\nonumber\\
   &\leq(t-t_c)m\eta^2 \frac{1}{d K}\sum_{i=1}^K   \sum_{t'=t_c}^{t-1} \left(\frac{2n^2}{d} m\sum_{r'=1}^m\left\|  \mathbf{W}_{r'}^{(i)}(t')  -\mathbf{W}_{r'}(t')   \right\|^2_{\mathrm{F}}    + 2n  \sum_{(\bm{x},y)\in S_i}\left\|   f(\mathbf{W}(t'),\bm{v},\bm{x}) - y   \right\|^2_{\mathrm{F}}\right)\nonumber\\
   &\leq(t-t_c)m\eta^2 \frac{1}{ dK}\sum_{i=1}^K   \sum_{t'=t_c}^{t-1} \left(\frac{2mn^2}{d}  \left\|  \mathbf{W}^{(i)}(t')  -\mathbf{W}(t')   \right\|^2_{\mathrm{F}}    + 2n  \sum_{(\bm{x},y)\in S_i}\left\|   f(\mathbf{W}(t'),\bm{v},\bm{x}) - y   \right\|^2_{\mathrm{F}}\right)\nonumber\\
    &\leq 2m^2n^2(t-t_c)\eta^2 \frac{1}{d^2 K}\sum_{i=1}^K   \sum_{t'=t_c}^{t-1} \left(  \left\|  \mathbf{W}^{(i)}(t')  -\mathbf{W}(t')   \right\|^2_{\mathrm{F}} \right) +\frac{4mn}{d} (t-t_c)\eta^2     \sum_{t'=t_c}^{t-1}  L(\mathbf{W}(t')),
\end{align*}
where \ding{192} and \ding{193} follows the Jensen's inequality.
Letting $a_t = \frac{1}{K}\sum_{i=1}^K     \left\|  \mathbf{W}^{(i)}(t)  -\mathbf{W}(t')   \right\|^2 $ and $b_t = L(\mathbf{W}(t))$, we can rewrite the above inequality as:
\begin{align*}
    a_t \leq \frac{2m^2n^2}{d^2} (t-t_c) \eta^2 \sum_{t'=t_c}^{t-1} a_{t'} + \frac{4mn}{d}  (t-t_c) \eta^2 \sum_{t'=t_c}^{t-1} b_{t'}. 
\end{align*}
Summing over $t$ from $t_c$ to $h$, where $t_c \leq h\leq t_c+\tau$ gives:

\begin{align*}
    \sum_{t=t_c}^{h} a_t &\leq  \sum_{t=t_c}^{h}\frac{2m^2n^2}{d^2} (t-t_c) \eta^2 \sum_{t'=t_c}^{t-1} a_{t'} +  \sum_{t=t_c}^{h}\frac{4mn}{d} (t-t_c) \eta^2 \sum_{t'=t_c}^{t-1} b_{t'}\nonumber\\
    &\leq  \sum_{t=t_c}^{h}\frac{2m^2n^2}{d^2} \tau \eta^2 \sum_{t'=t_c}^{t-1} a_{t'} +  \sum_{t=t_c}^{h}\frac{4mn}{d} \tau \eta^2 \sum_{t'=t_c}^{t-1} b_{t'}\nonumber\\
     &\leq  h \frac{2m^2n^2}{d^2} \tau \eta^2 \sum_{t'=t_c}^{h} a_{t'} +   h \frac{4mn}{d}  \tau \eta^2 \sum_{t'=t_c}^{h} b_{t'}\nonumber\\
     &\leq   \frac{2m^2n^2}{d^2} \tau^2 \eta^2 \sum_{t'=t_c}^{h} a_{t'} +    \frac{4mn}{d}  \tau^2 \eta^2 \sum_{t'=t_c}^{h} b_{t'}\nonumber\\
\end{align*}
Re-arranging the terms, and using the fact that $1-\frac{2m^2n^2\eta^2\tau^2 }{d^2}\geq \frac{1}{2}$ yields:

\begin{align*}
    \sum_{t=t_c}^{h} a_t  \leq     \frac{8mn}{d}   \tau^2 \eta^2 \sum_{t'=t_c}^{h} b_{t'}\nonumber.
\end{align*}
So, we can conclude that:
\begin{align*}
     a_t & \leq  \frac{2m^2n^2}{d^2} (t-t_c) \eta^2 \sum_{t'=t_c}^{t-1} a_{t'} +  \frac{4mn}{d}  (t-t_c) \eta^2 \sum_{t'=t_c}^{t-1} b_{t'}\nonumber\\
     &\leq  \frac{2m^2n^2}{d^2} \tau \eta^2 \sum_{t'=t_c}^{t-1} a_{t'} +  \frac{4mn}{d}  \tau \eta^2 \sum_{t'=t_c}^{t-1} b_{t'}\nonumber\\
     &\leq \left(\frac{16m^3n^3 \tau^3 \eta^4}{d^3}+ \frac{4mn\tau \eta^2}{d}\right) \sum_{t'=t_c}^{t-1} b_{t'}\nonumber.
\end{align*}
\end{proof}
\end{lemma}

The next lemma is the key result in our proof, which characterizes the semi gradient Lipschitzness property of ReLU neural network.     
 \begin{lemma}[Semi gradient Lipschitzness]\label{lm: gradient gap} For Local GD, at any iteration $t$, if $\mathbf{W}^{(i)}(t), \mathbf{W}(t) \in \mathcal{B}(\bm{W}(0),\omega)$, then with probability at least $1-\exp\left(-O(m\omega^{2/3})\right)$, the following statement holds true:
\begin{align*}
    \frac{1}{K}\sum_{i=1}^K \left\| \nabla_{\mathbf{W}^{(i)}}L_i(\mathbf{W}^{(i)}(t))- \nabla_{\mathbf{W} }L_i  (\mathbf{W}(t))\right\|^2_{\mathrm{F}} &\leq \frac{2 m^2n^2}{d^2}\frac{1}{K}\sum_{i=1}^K   \left\|   \mathbf{W}^{(i)}(t)    -     \mathbf{W}(t)   \right\|^2_{\mathrm{F}} \\
    & \quad+  \frac{C\omega^{2/3}  mn\log(m)}{d} L(\mathbf{W}(t)),
\end{align*}
where $K$ is the number of devices, $\tau$ is the number of local updates between two consecutive rounds of synchronization, $n$ is the size of each local data shard, and $m$ is the number of neurons in hidden layer.
\begin{proof}
\begin{align*}
   &\frac{1}{K}\sum_{i=1}^K \left\| \nabla_{\mathbf{W}^{(i)}}L_i(\mathbf{W}^{(i)}(t))- \nabla_{\mathbf{W} }L_i  (\mathbf{W}(t))\right\|^2_{\mathrm{F}} \nonumber\\
   & = \frac{1}{K}\sum_{i=1}^K  \left\| \nabla_{\mathbf{W}_r}L_i(\mathbf{W}^{(i)}(t))- \nabla_{\mathbf{W}_r }L_i  (\mathbf{W}(t))\right\|^2_{\mathrm{F}}\nonumber\\
   & = \frac{1}{K}\sum_{i=1}^K  \left\| \sum_{(\bm{x}_j,y_j)\in S_i}\left[ \mathbf{D}^{(i)}_j\bm{v} \left(f(\mathbf{W}^{(i)}(t),\bm{v},\bm{x}_j) - y_j \right)  \bm{x}_j^\top - \mathbf{D}_j \bm{v} \left(f(\mathbf{W}(t),\bm{v},\bm{x}_j) - y_j \right)  \bm{x}_j^\top \right] \right\|^2_{\mathrm{F}}\nonumber\\
   & \leq 2\frac{1}{K}\sum_{i=1}^K  \left\| \sum_{(\bm{x}_j,y_j)\in S_i}\left[ \mathbf{D}^{(i)}_j\bm{v}\left(f(\mathbf{W}^{(i)}(t),\bm{v},\bm{x}_j) - y_j \right)  - \left(f(\mathbf{W}(t),\bm{v},\bm{x}_j) - y_j \right)  \right]  \bm{x}_j^\top\right\|^2_{\mathrm{F}}\nonumber\\
     & \quad + 2\frac{1}{K}\sum_{i=1}^K  \left\| \sum_{(\bm{x}_j,y_j)\in S_i}   \left[\mathbf{D}^{(i)}_j\bm{v} - \mathbf{D}_j \bm{v} \right]\left(f(\mathbf{W}(t),\bm{v},\bm{x}_j) - y_j \right)\bm{x}_j^\top  \right\|^2_{\mathrm{F}}\nonumber\\
      & \stackrel{\text{\ding{192}}}{\leq} \frac{2m}{d}\frac{1}{K}\sum_{i=1}^K   n\sum_{(\bm{x}_j,y_j)\in S_i}\left\|  \bm{v}^\top \sigma(\mathbf{W}^{(i)}(t) \bm{x}_j) -   \bm{v}^\top \sigma(\mathbf{W}(t) \bm{x}_j) \right\|^2_{\mathrm{F}}\nonumber\\
      & \quad+ 2\frac{1}{K}\sum_{i=1}^K n\sum_{(\bm{x}_j,y_j)\in S_i}  \left\|    \left(f(\mathbf{W}(t),\bm{v},\bm{x}_j) - y_j \right)\right\|^2_{\mathrm{F}}\left\| (\mathbf{D}^{(i)}_j - \mathbf{D}_j) \bm{v}  \right\|^2\nonumber\\
      & \leq \frac{2 m^2n^2}{d^2}\frac{1}{K}\sum_{i=1}^K   \left\|   \mathbf{W}^{(i)}(t)    -     \mathbf{W}(t)   \right\|^2_{\mathrm{F}} +  \frac{C\omega^{2/3}  mn\log(m)}{d} L(\mathbf{W}(t))\nonumber,
\end{align*} 
where $ {\mathbf{D}}_{j}^{(i)}(r,r) = \sigma'(\langle \mathbf{W}_r^{(i)}(t), \bm{x}_j \rangle)$, $ {\mathbf{D}}_{j}(r,r) = \sigma'(\langle \mathbf{W}_r(t), \bm{x}_j \rangle)$ and \ding{192} follows the Jensen's inequality. Now, according to Lemma~\ref{lemma:perturbation}, we can upper bound $\left\| (\mathbf{D}^{(i)}_j - \mathbf{D}_j) \bm{v}  \right\|^2$ so that we conclude the proof:
\begin{align*}
   &\frac{1}{K}\sum_{i=1}^K \left\| \nabla_{\mathbf{W}^{(i)}}L_i(\mathbf{W}^{(i)}(t))- \nabla_{\mathbf{W} }L_i  (\mathbf{W}(t))\right\|^2_{\mathrm{F}} \nonumber\\ 
      & \leq \frac{2 m^2n^2}{d^2}\frac{1}{K}\sum_{i=1}^K   \left\|   \mathbf{W}^{(i)}(t)    -     \mathbf{W}(t)   \right\|^2_{\mathrm{F}} +  \frac{C\omega^{2/3}  mn\log(m)}{d} L(\mathbf{W}(t))\nonumber.
\end{align*} 
\end{proof}
\end{lemma}

 \subsection{Proof of Theorem~\ref{theorem: local GD}:}
With the key lemmas in place, we now  prove Theorem~\ref{theorem: local GD} by induction. Assume the following induction hypotheses hold for $h \leq t$:
 \begin{align}
      &\textbf{(I)} \quad \left \| \mathbf{W}(h) -  \mathbf{W}(0)\right\| \leq \omega,  \left \| \mathbf{W}^{(i)}(h) -  \mathbf{W}(0)\right\| \leq \omega, \quad \forall i \in [K]\nonumber, \\ 
      &\textbf{(II)} \quad L(\mathbf{W}(h))   \le\left(1-  \Omega\left(\frac{\eta m \phi}{dn^2}\right)\right)^{h} L( \mathbf{W}(0))\nonumber\\
      & \qquad \qquad \qquad \quad \quad +  \exp\left[{  O  \left(  \frac{  n^6     }{d^{1/2} \phi^{7/2} m^{1/2}   }\right)   } \right]O  \left(\frac{ m^{7/2}n^4 \tau^3 \eta^3}{\phi^{5/2} d^{7/2}}+ \frac{ m^{3/2}n^2 \tau \eta }{\phi^{5/2} d^{3/2}}\right)   L(\mathbf{W}(0))    \nonumber,  
 \end{align}
 where $\omega = O\big(\phi^{3/2} n^{-9} \log^{-3/2}(m)\big)$. Then we shall show the above two statements hold for $t+1$.
  \subsubsection{Proof of inductive hypothesis I}
  \paragraph{Step 1: Bounded virtual average iterates.}
  First we prove the first hypothesis for $t+1$: $\left \| \mathbf{W}(t+1) -  \mathbf{W}(0)\right\| \leq \omega $. By the updating rule we know that:
   \begin{align}
      \left \| \mathbf{W}(t+1) -  \mathbf{W}(0)\right\| &\leq \eta \sum_{j=1}^t\left \|\frac{1}{K}\sum_{i=1}^K \nabla L_i (\mathbf{W}^{(i)}(t))\right\| \nonumber\\
      &\leq \eta\sum_{j=1}^t \left \|\nabla L  (\mathbf{W}(t) )\right\| +\eta \frac{1}{K}\sum_{i=1}^K \left \|\nabla L_i (\mathbf{W}^{(i)}(t))-\nabla L_i  (\mathbf{W}(t) )\right\|\nonumber\\
       &= \eta\sum_{j=1}^t \left \|\nabla L  (\mathbf{W}(t) )\right\|_{\mathrm{F}} +\eta \frac{1}{K}\sum_{i=1}^K \sqrt{\left \|\nabla L_i (\mathbf{W}^{(i)}(t))-\nabla L_i  (\mathbf{W}(t) )\right\|^2_{\mathrm{F}}}.\nonumber
 \end{align}
 According to the concavity of $\sqrt{x}$ and Jensen's inequality, we have:
    \begin{align}
      \left \| \mathbf{W}(t+1) -  \mathbf{W}(0)\right\| & \leq \eta \sum_{j=1}^t\left \|\nabla L  (\mathbf{W}(j) )\right\|_{\mathrm{F}} + \eta \sqrt{\frac{1}{K}\sum_{i=1}^K \left \|\nabla L_i (\mathbf{W}^{(i)}(j))-\nabla L_i  (\mathbf{W}(j) )\right\|^2_{\mathrm{F}}}.\nonumber
 \end{align}
Plugging in results from Lemma~\ref{lemma: weight gap GD} and Lemma~\ref{lm: gradient gap} gives:
 
\begin{align*}
      &\left \| \mathbf{W}(t+1) -  \mathbf{W}(0)\right\| \\
      & \leq \eta\sum_{j=1}^t \left \|\nabla L  (\mathbf{W}(j) )\right\|_{\mathrm{F}} + \eta\sum_{j=1}^t\sqrt{ \frac{2 m^2n^2}{d^2}\frac{1}{K}\sum_{i=1}^K   \left\|   \mathbf{W}^{(i)}(j)  -\mathbf{W}(j)   \right\|^2_{\mathrm{F}} + \frac{C\omega^{2/3}  mn\log(m)}{d} L(\mathbf{W}(j)) }\nonumber\\
      & \leq \eta\sum_{j=1}^t \left \|\nabla L  (\mathbf{W}(j) )\right\|_{\mathrm{F}}\\
      & \quad +\eta \sum_{j=1}^t\sqrt{ \frac{2 m^2n^2}{d^2} \left(\left(\frac{16m^3n^3 \tau^3 \eta^4}{d^3}+ \frac{4mn\tau \eta^2}{d}\right)\sum_{t'=t_c}^{t-1} L(\mathbf{W}(t'))\right) + \frac{C\omega^{2/3}  mn\log(m)}{d}L(\mathbf{W}(j))}\nonumber. 
 \end{align*} 
 Applying the gradient upper bound (Lemma~\ref{lemma:grad bounds}) yields:
  
\begin{align}
      &\left \| \mathbf{W}(t+1) -  \mathbf{W}(0)\right\| \nonumber\\
      &  \leq \underbrace{\eta \sum_{j=1}^t O\big(\sqrt{mn L(\mathbf{W}(j))/ d}\big)}_{\spadesuit}\nonumber\\
      & \quad+ \underbrace{ \eta\sum_{j=1}^t\sqrt{ \frac{2 m^2n^2}{d^2} \left(\left(\frac{16m^3n^3 \tau^3 \eta^4}{d^2}+ \frac{4mn\tau \eta^2}{d}\right)\sum_{t'=t_c}^{t-1} L(\mathbf{W}(t'))\right) + \frac{C\omega^{2/3}  mn\log(m)}{d}L(\mathbf{W}(j))}}_{\heartsuit}\nonumber, 
 \end{align} 
 where $t_c$ is the latest communication round at iteration $j$. Now we will bound $\spadesuit$ and $\heartsuit$ separately.
 
 We first bound $\spadesuit$ as follows:
 \begin{align*}
     \spadesuit &\stackrel{\text{\ding{192}}}{=} \eta\sum_{j=1}^t O\big(\sqrt{m n /d}\big)\\
     &\quad \sqrt{\left(1-  \Omega\left(\frac{\eta m \phi}{dn^2}\right)\right)^{h} L( \mathbf{W}(0))  +   \exp\left[{  O  \left(  \frac{  n^6     }{d^{1/2} \phi^{7/2} m^{1/2}   }\right)   } \right]O  \left(\frac{ m^{7/2}n^4 \tau^3 \eta^3}{\phi^{5/2} d^{7/2}}+ \frac{ m^{3/2}n^2 \tau \eta }{\phi^{5/2} d^{3/2}}\right)    L(\mathbf{W}(0))  }\nonumber\\
     &\stackrel{\text{\ding{193}}}{\leq} \eta\sum_{j=1}^t O\big(\sqrt{m n /d}\big)\\
     &\quad\left(\sqrt{\left(1-  \Omega\left(\frac{\eta m \phi}{dn^2}\right)\right)^{j} L( \mathbf{W}(0))} +\sqrt{ \exp\left[{  O  \left(  \frac{  n^6     }{d^{1/2} \phi^{7/2} m^{1/2}   }\right)   } \right]O  \left(\frac{ m^{7/2}n^4 \tau^3 \eta^3}{\phi^{5/2} d^{7/2}}+ \frac{ m^{3/2}n^2 \tau \eta }{\phi^{5/2} d^{3/2}}\right)     L(\mathbf{W}(0))  }\right)\nonumber\\
     &\stackrel{\text{\ding{194}}}{\leq}  \eta O\big(\sqrt{m n /d}\big)\sum_{j=1}^t \left(1-  \Omega\left(\frac{\eta m \phi}{2dn^2 }\right)\right)^{j} \sqrt{L( \mathbf{W}(0))}\\
     &\quad+t\eta O\big(\sqrt{m n /d}\big)\sqrt{  \exp\left[{  O  \left(  \frac{  n^6     }{d^{1/2} \phi^{7/2} m^{1/2}   }\right)   } \right]O  \left(\frac{ m^{7/2}n^4 \tau^3 \eta^3}{\phi^{5/2} d^{7/2}}+ \frac{ m^{3/2}n^2 \tau \eta }{\phi^{5/2} d^{3/2}}\right)   L(\mathbf{W}(0))  } \nonumber\\
     &  \leq  \eta O\big(\sqrt{m n /d}\big)     O\left(\frac{2dn^2 }{\eta m \phi}\right) \sqrt{L( \mathbf{W}(0))}\\
     &\quad+t\eta O\big(\sqrt{m n /d}\big)\sqrt{  \exp\left[{  O  \left(  \frac{  n^6     }{d^{1/2} \phi^{7/2} m^{1/2}   }\right)   } \right]O  \left(\frac{ m^{7/2}n^4 \tau^3 \eta^3}{\phi^{5/2} d^{7/2}}+ \frac{ m^{3/2}n^2 \tau \eta }{\phi^{5/2} d^{3/2}}\right)   L(\mathbf{W}(0))  } \nonumber\\
      &\leq       O\left(\frac{\sqrt{d}n^{3/2} }{ \sqrt{m} \phi}\right) \sqrt{L( \mathbf{W}(0))}\\
      &\quad+t\eta O\big(\sqrt{m n /d}\big)\sqrt{ \exp\left[{  O  \left(  \frac{  n^6     }{d^{1/2} \phi^{7/2} m^{1/2}   }\right)   } \right]O  \left(\frac{ m^{7/2}n^4 \tau^3 \eta^3}{\phi^{5/2} d^{7/2}}+ \frac{ m^{3/2}n^2 \tau \eta }{\phi^{5/2} d^{3/2}}\right)   L(\mathbf{W}(0))  } \nonumber,
 \end{align*}
where in \ding{192} we plug in inductive hypothesis \textbf{II} to bound $L(\mathbf{W}(j))$, in \ding{193} we use the inequality $\sqrt{a+b} \leq \sqrt{a} + \sqrt{b}$, and in \ding{194} we use the fact $(1-a)^{1/2} \leq 1-\frac{a}{2}$. 

Recalling our choice of  $m \geq \frac{n^{21} (\log m)^3 d}{\phi^5}$, $\eta = \frac{d n^2\log T}{m\phi T}$ we have 
$$T \geq  \frac{  d^{1/2}n^{33/2}(\log T)^3(\log m)^{3/2} \tau }{     \phi^{5}} \exp\left( \frac{1 }{ \phi n^{9/2} (\log m)^{3/2}}\right) \geq \frac{d^{3/2} n^{27}   (\log T)^3 \tau(\log m)^{3 }}{m^{1/2} \phi^{15/2} }\exp\left[{  O  \left(  \frac{  n^6  }{ d^{1/2}\phi^{7/2} m^{1/2}   }\right)   } \right], $$
we conclude that $\spadesuit \leq \omega = O\big(\phi^{3/2}n^{-9} \log^{-3/2}(m)\big)$.
 
We now turn to bounding $\heartsuit$ as follows:
 \begin{align*}
     \heartsuit &=  \eta\sum_{j=1}^t\sqrt{ \frac{2 m^2n^2}{d^2} \left(\left(\frac{16m^3n^3 \tau^3 \eta^4}{d^3}+ \frac{4mn\tau \eta^2}{d}\right)\sum_{t'=t_c}^{t-1} L(\mathbf{W}(t'))\right) + \frac{C\omega^{2/3} mn\log (m)}{d}L(\mathbf{W}(j))}\nonumber\\
    &\leq  \eta \sqrt{ \frac{2 m^2n^2}{d^2} \left(\frac{16m^3n^3 \tau^3 \eta^4}{d^3}+ \frac{4mn\tau \eta^2}{d}\right)   }   \underbrace{\sum_{j=1}^t\sqrt{   \sum_{t'=t_c}^{j-1} L(\mathbf{W}(t')) }}_{T_1} +  \underbrace{\eta\sum_{j=1}^t\sqrt{\frac{C\omega^{2/3} mn\log (m)}{d}L(\mathbf{W}(j))}}_{T_2} \nonumber.
 \end{align*}
 We need to apply the bound for $L(\mathbf{W}(j))$ again, to bound $T_1$ and $T_2$. For $T_1$ we have:
 \begin{align*}
    & T_1 \\
    &= \sum_{j=1}^t\sqrt{   \sum_{t'=t_c}^{j-1} \left(\left(1-  \Omega\left(\frac{\eta m \phi}{dn^2}\right)\right)^{t'} L( \mathbf{W}(0))  +   \exp\left[{  O  \left(  \frac{  n^6     }{d^{1/2} \phi^{7/2} m^{1/2}   }\right)   } \right]O  \left(\frac{ m^{7/2}n^4 \tau^3 \eta^3}{\phi^{5/2} d^{7/2}}+ \frac{ m^{3/2}n^2 \tau \eta }{\phi^{5/2} d^{3/2}}\right)  L(\mathbf{W}(0))  \right)  } \nonumber\\
     & \leq \sum_{j=1}^t  \sum_{t'=t_c}^{j-1}\sqrt{  \left(1-  \Omega\left(\frac{\eta m \phi}{dn^2}\right)\right)^{t'} L( \mathbf{W}(0))} \\
     & \quad + t\sqrt{   \exp\left[{  O  \left(  \frac{  n^6     }{d^{1/2} \phi^{7/2} m^{1/2}   }\right)   } \right]O  \left(\frac{ m^{7/2}n^4 \tau^3 \eta^3}{\phi^{5/2} d^{7/2}}+ \frac{ m^{3/2}n^2 \tau \eta }{\phi^{5/2} d^{3/2}}\right) L(\mathbf{W}(0))   }    \nonumber\\
        & \leq \tau\sum_{j=1}^t\sqrt{    \left(1-  \Omega\left(\frac{\eta m \phi}{dn^2 }\right)\right)^{j} L( \mathbf{W}(0))} \\
        &\quad +  t\sqrt{  \exp\left[{  O  \left(  \frac{  n^6     }{d^{1/2} \phi^{7/2} m^{1/2}   }\right)   } \right]O  \left(\frac{ m^{7/2}n^4 \tau^3 \eta^3}{\phi^{5/2} d^{7/2}}+ \frac{ m^{3/2}n^2 \tau \eta }{\phi^{5/2} d^{3/2}}\right)  L(\mathbf{W}(0))   }    \nonumber\\
         & \leq \tau\sum_{j=1}^t    \left(1-  \Omega\left(\frac{\eta m \phi}{2dn^2 }\right)\right)^{j} \sqrt{L( \mathbf{W}(0))} \\
         & \quad +  t\sqrt{    \exp\left[{  O  \left(  \frac{  n^6     }{d^{1/2} \phi^{7/2} m^{1/2}   }\right)   } \right]O  \left(\frac{ m^{7/2}n^4 \tau^3 \eta^3}{\phi^{5/2} d^{7/2}}+ \frac{ m^{3/2}n^2 \tau \eta }{\phi^{5/2} d^{3/2}}\right)   L(\mathbf{W}(0))  }    \nonumber\\
           & \leq \tau O\left(\frac{2dn^2 }{\eta m \phi}\right)  \sqrt{L( \mathbf{W}(0))} \\
           & \quad +  t\sqrt{  \exp\left[{  O  \left(  \frac{  n^6     }{d^{1/2} \phi^{7/2} m^{1/2}   }\right)   } \right]O  \left(\frac{ m^{7/2}n^4 \tau^3 \eta^3}{\phi^{5/2} d^{7/2}}+ \frac{ m^{3/2}n^2 \tau \eta }{\phi^{5/2} d^{3/2}}\right)  L(\mathbf{W}(0))   }    \nonumber.
 \end{align*}

For $T_2$, we already know that $T_2  \leq O(\omega)$ when we bound $\spadesuit$. 
So we have
\begin{align*}
    \heartsuit &\leq \eta \sqrt{ \frac{2 m^2n^2}{d^2} \left(\frac{16m^3n^3 \tau^3 \eta^4}{d^3}+ \frac{4mn\tau \eta^2}{d}\right)   } \nonumber\\
    &\quad\left(\tau O\left(\frac{2dn ^2}{\eta m \phi}\right)  \sqrt{L( \mathbf{W}(0))} +  t\sqrt{  \exp\left[{  O  \left(  \frac{  n^6     }{d^{1/2} \phi^{7/2} m^{1/2}   }\right)   } \right]O  \left(\frac{ m^{7/2}n^4 \tau^3 \eta^3}{\phi^{5/2} d^{7/2}}+ \frac{ m^{3/2}n^2 \tau \eta }{\phi^{5/2} d^{3/2}}\right) L( \mathbf{W}(0))  } \right) +  O(\omega)\nonumber\\
    &\leq O\left(\frac{\tau^{3/2}m^{1/2}n^{7/2} \eta}{ d^{1/2}\phi}\right)+  O(\omega)\nonumber.
\end{align*}

According to our choice of $\eta$, $T$, $\tau$ and $m$, we know that:
\begin{align*}
    T\geq   \frac{\tau^{3/2}n^{4}\log T }{d^{1/2}\phi  (\log m)^{3/2} }  \geq \frac{\tau^{3/2}n^{29/2}d^{1/2}\log T (\log m)^{3/2}}{m^{1/2}\phi^{7/2}},
\end{align*}

we conclude that $\heartsuit\leq \omega$.
 \paragraph{Step 2: Bounded local iterates.} Now we verify the second statement in hypothesis (\textbf{I}), the boundedness of local iterates. For any $i \in [K]$, we have:
 \begin{align}
      \left \| \mathbf{W}^{(i)}(t+1) -  \mathbf{W}(0)\right\| & \leq \left \| \mathbf{W}^{(i)}(t+1) -  \mathbf{W}(t+1) \right\| + \left \| \mathbf{W}(t+1) -  \mathbf{W}(0)\right\|\nonumber. 
 \end{align}
 Since we know that $\left \| \mathbf{W}(t+1) -  \mathbf{W}(0)\right\| \leq O(\omega)$ from Step~1, then it remains to verify $\left\| \mathbf{W}^{(i)}(t+1) -  \mathbf{W}(t+1) \right\|\leq O(\omega)$. According to Lemma~\ref{lemma: weight gap GD}:
 \begin{align*}
    \left\| \mathbf{W}^{(i)}(t+1) -  \mathbf{W}(t+1) \right\| &\leq K \cdot \frac{1}{K}\sum_{i=1}^K \sqrt{\left\| \mathbf{W}^{(i)}(t) -  \mathbf{W}(t) \right\|^2_{\mathrm{F}}}\\
    &\leq K \cdot  \sqrt{\frac{1}{K}\sum_{i=1}^K\left\| \mathbf{W}^{(i)}(t) -  \mathbf{W}(t) \right\|^2_{\mathrm{F}}} \\
    &\leq K\sqrt{\left(\frac{16m^3n^3 \tau^3 \eta^4}{d^3}+ \frac{4mn\tau \eta^2}{d}\right)\sum_{t'=t_c}^{t-1} L(\mathbf{W}(t'))}.
 \end{align*}
 We plug in the bound of loss from hypothesis (\textbf{II}), and obtain:
  \begin{align*}
    &\left\| \mathbf{W}^{(i)}(t+1) -  \mathbf{W}(t+1) \right\| \\  
    &\leq K\sqrt{\left(\frac{16m^3n^3 \tau^3 \eta^4}{d^3}+ \frac{4mn\tau \eta^2}{d}\right)}\\
    &\quad\sqrt{\sum_{t'=t_c}^{t-1}\left[ \left(1-  \Omega\left(\frac{\eta m \phi}{dn^2}\right)\right)^{t'} L( \mathbf{W}(0))  +  \exp\left[{  O  \left(  \frac{  n^6     }{d^{1/2} \phi^{7/2} m^{1/2}   }\right)   } \right]O  \left(\frac{ m^{7/2}n^4 \tau^3 \eta^3}{\phi^{5/2} d^{7/2}}+ \frac{ m^{3/2}n^2 \tau \eta }{\phi^{5/2} d^{3/2}}\right)  L(\mathbf{W}(0)) \right]}\\
      &\leq K\sqrt{\left(\frac{16m^3n^3 \tau^3 \eta^4}{d^3}+ \frac{4mn\tau \eta^2}{d}\right)}\\
    & \quad\sqrt{\tau \left[  L( \mathbf{W}(0))  +  \exp\left[{  O  \left(  \frac{  n^6     }{d^{1/2} \phi^{7/2} m^{1/2}   }\right)   } \right]O  \left(\frac{ m^{7/2}n^4 \tau^3 \eta^3}{\phi^{5/2} d^{7/2}}+ \frac{ m^{3/2}n^2 \tau \eta }{\phi^{5/2} d^{3/2}}\right)  L(\mathbf{W}(0)) \right]}.
 \end{align*}
 Since we choose 
 \begin{align*}
     T \geq K \tau n \log T \geq \frac{\tau d^{1/2} n^{23/2} \log T (\log m)^{3/2}}{m^{1/2}\phi^{5/2}},
 \end{align*}
 we can conclude that $\left\| \mathbf{W}^{(i)}(t+1) -  \mathbf{W}(t+1) \right\| \leq O(\omega)$.

  \subsubsection{Proof of inductive hypothesis II}
  \paragraph{Step 1: One iteration analysis from Semi-smoothness.}
Now we proceed to prove that hypothesis \textbf{II} holds for $t+1$. The first step is to characterize how global loss changes in one iteration. We use the technique from standard smooth non-convex optimization, but notice that here we only have semi-smooth objective.  According to semi-smoothness (Lemma~\ref{lemma:semi_smooth}) and updating rule:
\begin{align*} 
&L(\mathbf{W}(t+1))\le L( \mathbf{W}(t)) + \left\langle \nabla L( \mathbf{W}(t)),   \mathbf{W}(t+1)-  \mathbf{W}(t)\right \rangle \notag\\
&\quad+ C'\sqrt{nL(\mathbf{W}(t))}\cdot\frac{\omega^{1/3}\sqrt{m\log(m)}}{\sqrt{d}}\cdot \|\mathbf{W}(t+1)-  \mathbf{W}(t)\| + \frac{C''nm}{d}\|\mathbf{W}(t+1)- \mathbf{W}(t)\|^2\\
&\le L( \mathbf{W}(t)) - \left\langle \nabla L( \mathbf{W}(t)),    \eta \frac{1}{K}\sum_{i=1}^K \nabla  L_i(\mathbf{W}^{(i)}(t)) \right \rangle \notag\\
&\quad+\eta C'\sqrt{nL(\mathbf{W}(t))}\cdot\frac{\omega^{1/3}\sqrt{m\log(m)}}{\sqrt{d}}\cdot \left\|\frac{1}{K}\sum_{i=1}^K \nabla  L_i(\mathbf{W}^{(i)}(t))\right \| + \eta^2\frac{C''nm}{d}\left\|\frac{1}{K}\sum_{i=1}^K \nabla  L_i(\mathbf{W}^{(i)}(t))\right\|^2 \\
&\stackrel{\text{\ding{192}}}{\leq} L( \mathbf{W}(t)) -  \frac{\eta}{2}\left\| \nabla L( \mathbf{W}(t)) \right\|^2_{\mathrm{F}} -\frac{\eta}{2} \left\| \frac{1}{K}\sum_{i=1}^K \nabla  L_i(\mathbf{W}^{(i)}(t)) \right \|^2_{\mathrm{F}} +\frac{\eta}{2} \left\| \nabla L( \mathbf{W}(t))-\frac{1}{K}\sum_{i=1}^K \nabla  L_i(\mathbf{W}^{(i)}(t)) \right \|^2_{\mathrm{F}}  \\
&\quad+\eta C'\sqrt{nL(\mathbf{W}(t))} \cdot\frac{\omega^{1/3}\sqrt{m\log(m)}}{2\sqrt{d}}\left( \left\|  \nabla  L(\mathbf{W}(t))\right \|_{\mathrm{F}}+\left\|\frac{1}{K}\sum_{i=1}^K \nabla  L_i(\mathbf{W}^{(i)}(t))-  \nabla  L(\mathbf{W}(t))\right \|_{\mathrm{F}}\right) \\
&\quad+ \eta^2 \frac{C''nm}{d}\left\|\frac{1}{K}\sum_{i=1}^K \nabla  L_i(\mathbf{W}^{(i)}(t))\right\|^2_{\mathrm{F}} \\
&\le L( \mathbf{W}(t)) -  \eta\left\| \nabla L( \mathbf{W}(t)) \right\|^2_{\mathrm{F}} -\left(\eta - \eta^2 \frac{C''nm}{d}\right) \left\| \frac{1}{K}\sum_{i=1}^K \nabla  L_i(\mathbf{W}^{(i)}(t)) \right \|^2_{\mathrm{F}}\\
& \quad +\eta \left\| \nabla L( \mathbf{W}(t))-\frac{1}{K}\sum_{i=1}^K \nabla  L_i(\mathbf{W}^{(i)}(t)) \right \|^2_{\mathrm{F}} +\eta C'\sqrt{nL(\mathbf{W}(t))} \cdot\frac{\omega^{1/3}\sqrt{m\log(m)}}{2\sqrt{d}}\left\|  \nabla  L(\mathbf{W}(t))\right \|_{\mathrm{F}}  \\
&\quad+\eta C' \cdot\frac{\omega^{1/3}\sqrt{m\log(m)}}{2\sqrt{d}}\left(  \left\| \nabla L( \mathbf{W}(t))-\frac{1}{K}\sum_{i=1}^K \nabla  L_i(\mathbf{W}^{(i)}(t)) \right \|_{\mathrm{F}} \sqrt{L( \mathbf{W}(t))}\right),   
\end{align*}
where in \ding{192} we use the identity $\langle \bm{a},\bm{b} \rangle =  \frac{1}{2}\|\bm{a} \|^2+\frac{1}{2}\| \bm{b}\|^2 - \frac{1}{2}\|\bm{a}-\bm{b}\|^2$. 
We plug in the result from Lemma~\ref{lm: gradient gap}  in last inequality, and use the fact that $\eta - \eta^2 \frac{C''nm}{d} \geq 0$ to get:

\begin{align*} 
L(\mathbf{W}(t+1))  
&\le L( \mathbf{W}(t)) -  \eta\left\| \nabla L( \mathbf{W}(t)) \right\|^2_{\mathrm{F}}  +\eta C'\sqrt{nL(\mathbf{W}(t))} \cdot\frac{\omega^{1/3}\sqrt{m\log(m)}}{2\sqrt{d}}\left\|  \nabla  L(\mathbf{W}(t))\right \|_{\mathrm{F}}  \\
& \quad+\eta \left( \frac{2 m^2n^2}{d^2}\frac{1}{K}\sum_{i=1}^K   \left\|   \mathbf{W}^{(i)}(t)  -  \mathbf{W}(t)   \right\|^2_{\mathrm{F}} +  \frac{C\omega^{2/3}  m\log(m)}{d} L(\mathbf{W}(t)) \right )\notag\\
& \quad+\eta C' \cdot\frac{\omega^{1/3}\sqrt{m\log(m)}}{2\sqrt{d}}\\
&\quad\times\left(  \sqrt{\frac{2 m^2n^2}{d^2}\frac{1}{K}\sum_{i=1}^K   \left\|   \mathbf{W}^{(i)}(t)    -     \mathbf{W}(t)   \right\|^2_{\mathrm{F}} +  \frac{C\omega^{2/3}  m\log(m)}{d} L(\mathbf{W}(t))} \sqrt{L( \mathbf{W}(t))}\right).   
\end{align*}
Applying inequality $\sqrt{a+b} \leq \sqrt{a} + \sqrt{b} $ to split the square root, and choosing $\omega = \frac{ \phi^{3/2} }{C_\omega n^{9}\log(m)^{3/2}}$ where $C_\omega$ is some large constant yields:
\begin{align*} 
L(\mathbf{W}(t+1))  
&\le L( \mathbf{W}(t)) -  \eta\left\| \nabla L( \mathbf{W}(t)) \right\|^2_{\mathrm{F}} +\eta C'\sqrt{nL(\mathbf{W}(t))} \cdot\frac{\omega^{1/3}\sqrt{m\log(m)}}{2\sqrt{d}}\left\|  \nabla  L(\mathbf{W}(t))\right \|_{\mathrm{F}}  \\
& \quad  +\eta \left(\frac{2 m^2n^2}{d^2}\frac{1}{K}\sum_{i=1}^K   \left\|   \mathbf{W}^{(i)}(t)    -     \mathbf{W}(t)   \right\|^2_{\mathrm{F}} +  \frac{C\omega^{2/3}  mn\log(m)}{d} L(\mathbf{W}(t))   \right ) \notag\\
&\quad +\eta C' \cdot\frac{\omega^{1/3}\sqrt{m\log(m)}}{2\sqrt{d}}\\
&\left(  \sqrt{\frac{2 m^2n^2}{d^2}\frac{1}{K}\sum_{i=1}^K   \left\|   \mathbf{W}^{(i)}(t)    -     \mathbf{W}(t)   \right\|^2_{\mathrm{F}} } + \sqrt{\frac{C\omega^{2/3}  mn\log(m)}{d} L(\mathbf{W}(t)) } \right)\sqrt{L( \mathbf{W}(t))}\nonumber\\
&\le L( \mathbf{W}(t)) -  \eta\left\| \nabla L( \mathbf{W}(t)) \right\|^2_{\mathrm{F}} +\eta C'\sqrt{nL(\mathbf{W}(t))} \cdot\frac{\omega^{1/3}\sqrt{m\log(m)}}{2\sqrt{d}}\left\|  \nabla  L(\mathbf{W}(t))\right \|_{\mathrm{F}}  \\
&  \quad +\eta \left( \frac{2 m^2n^2}{d^2}\frac{1}{K}\sum_{i=1}^K   \left\|   \mathbf{W}^{(i)}(t)    -     \mathbf{W}(t)   \right\|^2_{\mathrm{F}} +  \frac{C\omega^{2/3}  mn\log(m)}{d} L(\mathbf{W}(t))   \right ) \notag\\
& \quad+\eta C' \cdot\frac{\omega^{2/3} m\log(m)\sqrt{Cn}}{ 2d }  L( \mathbf{W}(t)) \nonumber\\
& \quad+\eta C' \cdot\frac{\omega^{1/3}\sqrt{m\log(m)}}{4\sqrt{d}}\left(  \frac{2 m^2n^2}{d^2}\frac{1}{K}\sum_{i=1}^K   \left\|   \mathbf{W}^{(i)}(t)   -    \mathbf{W}(t)   \right\|^2_{\mathrm{F}}  + L( \mathbf{W}(t))  \right).
\end{align*}
We plug in gradient  bound from Lemma~\ref{lemma:grad bounds} and local model deviation bound from Lemma~\ref{lemma: weight gap GD},   to  get the main recursion relation as follows:
\begin{align} 
L(\mathbf{W}(t+1))  
&\le \left(1-  \Omega\left(\frac{\eta m \phi}{dn^2}\right)\right)L( \mathbf{W}(t)) \nonumber\\
& \quad + O\left(  \frac{ \eta m^2n^2}{d^2} +   \frac{\eta m^{5/2} }{\phi^{1/2}d^{5/2}n}    \right)\left(   \left(\frac{16m^3n^3 \tau^3 \eta^4}{d^3}+ \frac{4mn\tau \eta^2}{d}\right)\sum_{t'=t_c}^{t-1} L(\mathbf{W}(t'))   \right)  \nonumber \\
&\le \left(1-  \Omega\left(\frac{\eta m \phi}{dn^2}\right)\right)L( \mathbf{W}(t))  +  O  \left(\frac{ m^{11/2}n^2 \tau^3 \eta^5}{\phi^{1/2}d^{11/2}}+ \frac{ m^{7/2}\tau \eta^3}{\phi^{1/2}d^{7/2}}\right)\sum_{t'=t_c}^{t-1} L(\mathbf{W}(t'))    \label{eq: proof_GD_1}
\end{align}
 \paragraph{Step 2: Reducing cumulative loss to loss at communication round.}
 We then need to bound $\sum_{t'=t_c}^{t-1} L(\mathbf{W}(t')) $, which is the cumulative losses  between two communication rounds. We handle it by summing above inequality over $t$ from $t_c$ to $h$, where $t_c \leq h\leq t_c+\tau$:
  
\begin{align*} 
\sum_{t=t_c}^h L(\mathbf{W}(t+1))  
&\le\left(1-  \Omega\left(\frac{\eta m \phi}{dn^2}\right)\right)\sum_{t=t_c}^h L( \mathbf{W}(t))  + O\left(\frac{ m^{11/2}n^2 \tau^3 \eta^5}{\phi^{1/2}d^{11/2}}+ \frac{m^{7/2} \tau \eta^3}{\phi^{1/2}d^{7/2}}\right)\sum_{t=t_c}^h \sum_{t'=t_c}^{t-1} L(\mathbf{W}(t')) .
\end{align*}  
The LHS of above inequality can be equivalently written as:  
  \begin{align*} 
\sum_{t=t_c+1}^{h+1} L(\mathbf{W}(t))  
&\le\left(1-  \Omega\left(\frac{\eta m \phi}{dn^2}\right)\right)\sum_{t=t_c}^h L( \mathbf{W}(t))  +  \left(\frac{ m^{11/2}n^2 \tau^3 \eta^5}{\phi^{1/2}d^{11/2}}+ \frac{m^{7/2} \tau \eta^3}{\phi^{1/2}d^{7/2}}\right)\sum_{t=t_c}^h \sum_{t'=t_c}^{t-1} L(\mathbf{W}(t')) \nonumber\\
&\le\left(1-  \Omega\left(\frac{\eta m \phi}{dn^2}\right)\right)\sum_{t=t_c+1}^{h+1} L( \mathbf{W}(t)) + \left(1-  \Omega\left(\frac{\eta m \phi}{dn^2}\right)\right)  L( \mathbf{W}(t_c))\nonumber\\
&\quad +O\left(\frac{ m^{11/2}n^2 \tau^3 \eta^5}{\phi^{1/2}d^{11/2}}+ \frac{m^{7/2} \tau \eta^3}{\phi^{1/2}d^{7/2}}\right)h\sum_{t'=t_c}^{h} L(\mathbf{W}(t')). \nonumber\\
\end{align*}

Re-arranging the terms yields:
 \begin{align*} 
\Omega\left(\frac{\eta m \phi}{dn^2}\right)\sum_{t=t_c+1}^{h+1} L(\mathbf{W}(t))  
&\le \left(1-  \Omega\left(\frac{\eta m \phi}{dn^2}\right)\right)L(\mathbf{W}(t_c))+ O\left(\frac{ m^{11/2}n^2 \tau^3 \eta^5}{\phi^{1/2}d^{11/2}}+ \frac{m^{7/2}  \tau \eta^3}{\phi^{1/2}d^{7/2}}\right)h\sum_{t'=t_c}^{h} L(\mathbf{W}(t')) \nonumber.
\end{align*}
Dividing both sides with $\Omega\left(\frac{\eta m \phi}{dn^2}\right)$ gives:

 \begin{align*} 
 \sum_{t=t_c+1}^{h+1} L(\mathbf{W}(t)) 
&\le O\left(\frac{dn^2}{\eta m \phi}\right)L(\mathbf{W}(t_c))+  O\left(\frac{ m^{9/2}n^4 \tau^3 \eta^4}{\phi^{3/2} d^{9/2}}+ \frac{m^{5/2}n^2 \tau \eta^2}{\phi^{3/2} d^{5/2}}\right) h\sum_{t'=t_c}^{h} L(\mathbf{W}(t')) \nonumber.
\end{align*}
Expanding the LHS yields:

 \begin{align*} 
 \sum_{t=t_c}^{h} L(\mathbf{W}(t)) + L(\mathbf{W}(h+1)) -L(\mathbf{W}(t_c))
&\le O\left(\frac{dn^2}{\eta m \phi}\right)L(\mathbf{W}(t_c))\\
& \quad + O\left(\frac{ m^{9/2}n^4 \tau^3 \eta^4}{\phi^{3/2} d^{9/2}}+ \frac{m^{5/2}n^2 \tau \eta^2}{\phi^{3/2} d^{5/2}}\right)\tau\sum_{t'=t_c}^{h} L(\mathbf{W}(t')) \nonumber.
\end{align*}
Finally we can conclude the upper bound of $ \sum_{t=t_c}^{h} L(\mathbf{W}(t)) $: 
 \begin{align*} 
 \sum_{t=t_c}^{h} L(\mathbf{W}(t))  
&\leq \frac{O\left(\frac{dn^2}{\eta m \phi}\right)}{ \Omega\left( 1- (\frac{ m^{9/2}n^4 \tau^3 \eta^4}{\phi^{3/2} d^{9/2}}+ \frac{m^{5/2}n^2 \tau \eta^2}{\phi^{3/2} d^{5/2}}) \tau \right)} L(\mathbf{W}(t_c)).  
\end{align*}
According to our choice of $m$, $\tau$ and $\eta$, we have  $\frac{1}{ \Omega\left( 1- (\frac{ m^{9/2}n^5 \tau^3 \eta^4}{\phi^{3/2} d^{9/2}}+ \frac{m^{5/2}n^3 \tau \eta^2}{\phi^{3/2} d^{5/2}}) \tau \right)} = O(1)$. So we conclude:
\begin{align*} 
L(\mathbf{W}(t+1))   
&\le \left(1-  \Omega\left(\frac{\eta m \phi}{dn^2}\right)\right)L( \mathbf{W}(t))  +  O  \left(\frac{ m^{11/2}n^2 \tau^3 \eta^5}{\phi^{1/2}d^{11/2}}+ \frac{ m^{7/2}  \tau \eta^3}{\phi^{1/2}d^{7/2}}\right)O\left(\frac{dn ^2}{\eta m \phi}\right) L(\mathbf{W}(t_c))     \\
&\le \left(1-  \Omega\left(\frac{\eta m \phi}{dn^2}\right)\right)L( \mathbf{W}(t))  +  O  \left(\frac{ m^{9/2}n^4 \tau^3 \eta^4}{\phi^{3/2} d^{9/2}}+ \frac{ m^{5/2}n^2 \tau \eta^2}{\phi^{3/2} d^{5/2}}\right) L(\mathbf{W}(t_c)),  
\end{align*}

where $t_c$ is the latest communication round  of $t$, also the $c$-th communication round. 
 \paragraph{Step 3: Bounded loss at communication rounds.}
It remains to bound $L(\mathbf{W}(t_c))$, the objective value at communication round. We handle it by summing above inequality over $t $ from $t_{c}$ to $t_{c-1}$: 
\begin{align*} 
 L(\mathbf{W}(t_{c}))   
&\le  \left(1-  \Omega\left(\frac{\eta m \phi}{dn^2 }\right)\right)^\tau L( \mathbf{W}(t_{c-1}))\nonumber\\
& \quad +    \sum_{j=1}^\tau \left(1-  \Omega\left(\frac{\eta m \phi}{dn^2 }\right)\right)^j O  \left(\frac{ m^{9/2}n^4 \tau^3 \eta^4}{\phi^{3/2} d^{9/2}}+ \frac{ m^{5/2}n^2 \tau \eta^2}{\phi^{3/2} d^{5/2}}\right) L(\mathbf{W}(t_c))  \nonumber \\
&\le  \left[\left(1-  \Omega\left(\frac{\eta m \phi}{dn^2 }\right)\right)^\tau   +  O  \left(\frac{ m^{9/2}n^4 \tau^3 \eta^4}{\phi^{3/2} d^{9/2}}+ \frac{ m^{5/2}n^2 \tau \eta^2}{\phi^{3/2} d^{5/2}}\right)\tau\right] L(\mathbf{W}(t_{c-1}))  \nonumber \\
&\le  \left[\left(1-  \Omega\left(\frac{\eta m \phi}{dn^2 }\right)\right)^\tau   + O  \left(\frac{ m^{9/2}n^4 \tau^4 \eta^4}{\phi^{3/2} d^{9/2}}+ \frac{ m^{5/2}n^2 \tau^2 \eta^2}{\phi^{3/2} d^{5/2}}\right) \right]^c L(\mathbf{W}(0))  \nonumber. 
\end{align*}
Plugging in $\eta = \frac{d n^2\log T}{m\phi T}$, and letting $T = S\tau$ we have:
\begin{align*} 
 L(\mathbf{W}(t_{c+1}))   
&\le  \left[O\left(\frac{1}{T}\right)^{\frac{1}{S}}   +    O  \left(\frac{   m^{1/2}n^{12} \tau^4    (\log T)^4}{d^{1/2} \phi^{11/2}    T^4}+ \frac{  m^{1/2}  n^6 \tau^2  (\log T)^2 }{d^{1/2} \phi^{7/2}     T^2}\right)  \right]^c L(\mathbf{W}(0))  \nonumber  \\ 
&=  \left(O\left(\frac{1}{T}\right)^{\frac{1}{S}} \right)^c\left[1   +   O  \left(\frac{m^{1/2}   n^{12} \tau^4    (\log T)^4}{d^{1/2} \phi^{11/2}      T^{4-1/S}}+ \frac{ m^{1/2}  n^6 \tau^2  (\log T)^2 }{d^{1/2} \phi^{7/2}     T^{2-1/S}}\right) \right]^c L(\mathbf{W}(0))  \nonumber \\
&\stackrel{\text{\ding{192}}}{\leq}  \left[1   +    O  \left(  \frac{  n^6      }{d^{1/2}\phi^{7/2} m^{1/2}    S}\right)    \right]^S L(\mathbf{W}(0))  \nonumber \\
&\leq \left[1   +    O  \left(  \frac{  n^6     }{d^{1/2} \phi^{7/2} m^{1/2}    S}\right)    \right]^{ O  \left(  \frac{d^{1/2}\phi^{7/2} m^{1/2}    S}{  n^6      }\right)  O  \left(  \frac{  n^6     }{ d^{1/2}\phi^{7/2} m^{1/2}   }\right)   } L(\mathbf{W}(0))  \nonumber \\
&\leq   \exp\left[{  O  \left(  \frac{  n^6     }{d^{1/2} \phi^{7/2} m^{1/2}   }\right)   } \right]L(\mathbf{W}(0))  \nonumber,
\end{align*}
where in $\text{\ding{192}}$ we apply the inequality that:$ \frac{\tau^2 (\log T)^2}{T^{2-\frac{1}{S}}} \leq \frac{1}{Sm}$, which is realized by our choice of  $\tau \leq \frac{T^{1-1/S}}{m(\log T)^2}$.
Actually, this condition can be realized if we set $\tau = O(\sqrt{T/K})$ and $T^{1-\sqrt{T/K}} \geq m (\log T)^2 \sqrt{T/K}$ which is exactly the choice in Corollary~\ref{coro: GD}.
 
 \paragraph{Step 4: Sub-linear convergence of global loss.}
 Now we can finally bound $L(\mathbf{W}(t+1)) $ by plugging in the bound for $L(\mathbf{W}(t_c))$ and unrolling the recursion in (\ref{eq: proof_GD_1}) to get: 
\begin{align*} 
L(\mathbf{W}(t+1))   
&\le\left(1-  \Omega\left(\frac{\eta m \phi}{dn^2}\right)\right)^{t+1} L( \mathbf{W}(0))\\
& \quad +   \exp\left[{  O  \left(  \frac{  n^6     }{d^{1/2} \phi^{7/2} m^{1/2}   }\right)   } \right]O  \left(\frac{ m^{11/2}n^2 \tau^3 \eta^5}{\phi^{1/2}d^{11/2}}+ \frac{ m^{7/2}\tau \eta^3}{\phi^{1/2}d^{7/2}}\right) \sum_{j=1}^t \left(1-  \Omega\left(\frac{\eta m \phi}{dn^2}\right)\right)^j  L(\mathbf{W}(0))  \nonumber\\ 
 & \le\left(1-  \Omega\left(\frac{\eta m \phi}{dn^2}\right)\right)^{t+1} L( \mathbf{W}(0))\nonumber\\
 & \quad +  \exp\left[{  O  \left(  \frac{  n^6     }{d^{1/2} \phi^{7/2} m^{1/2}   }\right)   } \right]O \left(\frac{ m^{9/2}n^2 \tau^3 \eta^4}{\phi^{3/2} d^{9/2}}+ \frac{ m^{5/2}  \tau \eta^2}{\phi^{3/2} d^{5/2}}\right) O\left(\frac{dn^2}{\eta m \phi}\right)     L(\mathbf{W}(0))  \nonumber\\
  & \le\left(1-  \Omega\left(\frac{\eta m \phi}{dn^2}\right)\right)^{t+1} L( \mathbf{W}(0)) \\
  & \quad +   \exp\left[{  O  \left(  \frac{  n^6     }{d^{1/2} \phi^{7/2} m^{1/2}   }\right)   } \right]O  \left(\frac{ m^{7/2}n^4 \tau^3 \eta^3}{\phi^{5/2} d^{7/2}}+ \frac{ m^{3/2}n^2 \tau \eta }{\phi^{5/2} d^{3/2}}\right)   L(\mathbf{W}(0))  \nonumber.
\end{align*}
\qed
\section{Proof of Theorem~\ref{theorem: local SGD} (Local SGD)}\label{app: SGD}
In this section  we will present the proof of convergence rate of Local SGD (Theorem~\ref{theorem: local SGD}). Before that, let us first introduce some useful lemmas. 
\subsection{Proof of Technical Lemma}
The following lemma establishes the boundedness of variance, of the stochastic gradient.
\begin{lemma}[Bounded stochastic gradient]\label{lemma: bounded variance}
For Local SGD, the following statement holds true for stochastic gradient at any iteration $t$:
\begin{align*}
    \mathbb{E}_{S_t}\left[ \left \| \frac{1}{K}\sum_{i=1}^K \mathbf{G}_i^{(t)}  \right\|^2 \right] \leq  \frac{2m^2n^2}{d^2}\frac{1}{ K^2}\sum_{i=1}^K\left \|  \mathbf{W}^{(i)}(t)  -  \mathbf{W}(t) \right\|^2  +   \frac{2mn}{dK}L(\mathbf{W} (t) ).
\end{align*}
where $S_t = \{(\tilde{\bm{x}}_i, \tilde{y}_i)\}_{i=1}^K$ are the set of randomly sampled data to compute $\frac{1}{K}\sum_{i=1}^K \mathbf{G}_i^{(t)}$, $K$ is the number of devices, $\tau$ is the number of local updates between two consecutive rounds of synchronization, $n$ is the size of each local data shard, $d$ is the dimension of input data, and $m$ is the number of neurons in hidden layer.
\begin{proof}
\begin{align*}
    &\mathbb{E}_{S_t}\left[ \left \|\frac{1}{K}\sum_{i=1}^K \mathbf{G}_i^{(t)} \right\|^2 \right] \\
    &= \frac{1}{K^2}\sum_{i=1}^K\mathbb{E}\left[ \left \| n\nabla \ell (\mathbf{W}^{(i)}(t); \tilde{\bm{x}}_i, \tilde{y}_i)  \right\|^2 \right]\\
   & \leq \frac{1}{K}\sum_{i=1}^K\frac{1}{n}\sum_{( \bm{x}_j , y_j)\in S_i} \left \|n \nabla \ell (\mathbf{W}^{(i)}(t); \bm{x}_j , y_j)   \right\|^2    \\
     & = \frac{1}{K^2}\sum_{i=1}^K\frac{1}{n}\sum_{(\bm{x}_j,  y_j)\in S_i} n^2\sum_{r=1}^m\left \| \mathbf{D}^{(i)}_j \bm{v} \left(f(\mathbf{W}^{(i)}(t),\bm{v},\bm{x}_j) -  y_j\right)  \bm{x}_j    \right\|^2   \\
      & = \frac{1}{dK^2}\sum_{i=1}^K mn\sum_{(\bm{x}_j , y_j)\in S_i}  \left \|    \left(f(\mathbf{W}^{(i)}(t),\bm{v},\bm{x}_j) -  y_j\right)   \right\|^2   \\
      & = \frac{1}{dK^2}\sum_{i=1}^K mn\sum_{(\bm{x}_j , y_j)\in S_i} \left(2\left \| f(\mathbf{W}^{(i)}(t),\bm{v},\bm{x}_j) - f(\mathbf{W}(t),\bm{v},\bm{x}_j)\right\|^2  + 2\left \|f(\mathbf{W} (t),\bm{v},\bm{x}_j)  -  y_j \right\|^2 \right) \\
      & = \frac{1}{dK^2}\sum_{i=1}^K mn\sum_{(\bm{x}_j , y_j)\in S_i} \left(\frac{2m}{d}\left \|  \mathbf{W}^{(i)}(t)  -  \mathbf{W}(t) \right\|^2  + 2 \ell(\mathbf{W} (t) ,\bm{x}_j , y_j)  \right) \\
      & =   \frac{1}{ K^2}\sum_{i=1}^K\frac{2m^2n^2}{d^2}\left \|  \mathbf{W}^{(i)}(t)  -  \mathbf{W}(t) \right\|^2  +   \frac{2mn}{dK}L(\mathbf{W} (t) ).
\end{align*}
\end{proof}
\end{lemma}

The next lemma is the semi gradient Lipschitzness property of loss function, at the single data point. The significance of it is that even in the stochastic setting, where we only evaluate gradient on a randomly sampled subset of data points, the semi gradient Lipschitzness property still holds.

 \begin{lemma}[Semi gradient Lipschitzness at single point]\label{lm: one point gradient gap} For Local SGD, given a randomly sampled data pairs $(\tilde{\bm{x}}_i, \tilde{y}_i)$ from $ S_i$, if $\mathbf{W}^{(i)}(t), \mathbf{W}(t) \in \mathcal{B}(\bm{W}(0),\omega)$, then with probability at least $1-\exp\left(-O(m\omega^{2/3})\right)$ and for any $t$, the following statements hold true:
\begin{align*}
    \frac{1}{K}\sum_{i=1}^K \left\| n\nabla_{\mathbf{W}^{(i)}}\ell(\mathbf{W}^{(i)}(t);\tilde{\bm{x}}_i, \tilde{y}_i)- n\nabla_{\mathbf{W} }\ell (\mathbf{W}(t);\tilde{\bm{x}}_i, \tilde{y}_i)\right\|^2_{\mathrm{F}} & \leq\frac{ 2m^2n^2}{d^2 }\frac{1}{K}\sum_{i=1}^K   \left\|   \mathbf{W}^{(i)}(t)    -     \mathbf{W}(t)   \right\|^2_{\mathrm{F}} \\
    & \quad +  \frac{2\omega^{2/3}mn^2}{d}  L(\mathbf{W}(t)), 
\end{align*}
where $K$ is the number of devices, $\tau$ is the number of local updates between two consecutive rounds of synchronization, $d$ is the dimension of input data, and $m$ is the number of neurons in hidden layer.
\begin{proof}
According to the structure of gradient, we have:
\begin{align*}
   &\frac{1}{K}\sum_{i=1}^K \left\| n\nabla_{\mathbf{W}^{(i)}}\ell(\mathbf{W}^{(i)}(t);\tilde{\bm{x}}_{i}, \tilde{y}_{i})- n\nabla_{\mathbf{W} }\ell  (\mathbf{W}(t);\tilde{\bm{x}}_{i}, \tilde{y}_{i})\right\|^2_{\mathrm{F}} \nonumber\\ 
   & = \frac{1}{K}\sum_{i=1}^K  n^2\left\| \mathbf{D}^{(i)}\bm{v}  \left(f(\mathbf{W}^{(i)}(t),\bm{v},\tilde{\bm{x}}_{i}) - \tilde{y}_{i} \right)  \tilde{\bm{x}}_{i}  - \mathbf{D} \bm{v} \left(f(\mathbf{W}(t),\bm{v},\tilde{\bm{x}}_{i}) - \tilde{y}_{i} \right)  \tilde{\bm{x}}_{i}    \right\|^2_{\mathrm{F}}\nonumber\\
    & = \frac{1}{K}\sum_{i=1}^K  2 n^2\left\| \mathbf{D}^{(i)}\bm{v}  \left(f(\mathbf{W}^{(i)}(t),\bm{v},\tilde{\bm{x}}_{i}) - \tilde{y}_{i} \right)  \tilde{\bm{x}}_{i}  - \mathbf{D}^{(i)} \bm{v} \left(f(\mathbf{W}(t),\bm{v},\tilde{\bm{x}}_{i}) - \tilde{y}_{i} \right)  \tilde{\bm{x}}_{i}    \right\|^2_{\mathrm{F}}\nonumber\\
    & \quad +\frac{1}{K}\sum_{i=1}^K  2 n^2\left\| \mathbf{D}^{(i)}\bm{v}  \left(f(\mathbf{W} (t),\bm{v},\tilde{\bm{x}}_{i}) - \tilde{y}_{i} \right)  \tilde{\bm{x}}_{i}  - \mathbf{D} \bm{v} \left(f(\mathbf{W}(t),\bm{v},\tilde{\bm{x}}_{i}) - \tilde{y}_{i} \right)  \tilde{\bm{x}}_{i}    \right\|^2_{\mathrm{F}}\nonumber\\
    &\leq \frac{1}{K}\sum_{i=1}^K  \frac{2m n^2}{d}\left\| f(\mathbf{W}^{(i)}(t),\bm{v},\tilde{\bm{x}}_{i})  -   f(\mathbf{W}(t),\bm{v},\tilde{\bm{x}}_{i})    \right\|^2_{\mathrm{F}}  +\frac{1}{K}\sum_{i=1}^K  2 n^2\left\| \mathbf{D}^{(i)}\bm{v} - \mathbf{D} \bm{v} \right\|^2\left\| f(\mathbf{W}(t),\bm{v},\tilde{\bm{x}}_{i}) - \tilde{y}_{i} \right\|^2_{\mathrm{F}}\nonumber\\
    &\leq  \frac{2m^2 n^2}{d^2}\frac{1}{K}\sum_{i=1}^K \left\|  \mathbf{W}^{(i)}(t)   -   \mathbf{W}(t)    \right\|^2_{\mathrm{F}}  +\frac{2\omega^{2/3}mn^2}{d} L(\mathbf{W}(t))\nonumber.
\end{align*}

\end{proof}
\end{lemma}

The next lemma is similar to Lemma~\ref{lemma: weight gap GD}, but it characterizes the local model deviation under stochastic setting. Hence, it will be inevitably looser than the deterministic version (Lemma~\ref{lemma: weight gap GD}).  
\begin{lemma}\label{lemma: weight gap SGD non expectation}
For Local SGD, let $t_c$ is the latest communication stage before iteration $t$, the following statement holds true:
\begin{align*}
  \frac{1}{K}\sum_{i=1}^K \left\| \mathbf{W}^{(i)}(t) -  \mathbf{W}(t) \right\|^2_{\mathrm{F}} \leq\left(  \frac{16m^3n^4 \tau^3 \eta^4}{d^3}+ \frac{4m n^2}{ d} \tau \eta^2\right) \sum_{t'=t_c}^{t-1}  L(\mathbf{W}(t')),
\end{align*}
where $K$ is the number of devices, $\tau$ is the number of local updates between two consecutive rounds of synchronization, $n$ is the size of each local data shard, $d$ is the dimension of input data, and $m$ is the number of neurons in hidden layer.
\begin{proof}
 According our updating rule in Local SGD, we have:
\begin{align*}
 &\frac{1}{K}\sum_{i=1}^K \left\| \mathbf{W}^{(i)}(t) -  \mathbf{W}(t) \right\|^2_{\mathrm{F}}  \nonumber\\
 &\leq \eta^2 \frac{1}{K}\sum_{i=1}^K   \left\|  \sum_{t'=t_c}^{t-1}\left( \mathbf{G}_i^{(t)} -   \frac{1}{K}\sum_{j=1}^K  \mathbf{G}_j^{(t)} \right)\right\|^2_{\mathrm{F}} \\
&\leq (t-t_c)\eta^2 \frac{1}{K}\sum_{i=1}^K \sum_{t'=t_c}^{t-1}  \left\|  n  \nabla_{\mathbf{W}^{(i)}} \ell (\mathbf{W}^{(i)}(t'); \tilde{\bm{x}}_i, \tilde{y}_i) -   n\frac{1}{K}\sum_{j=1}^K \nabla_{\mathbf{W}^{(j)}}\ell (\mathbf{W}^{(j)}(t') ; \tilde{\bm{x}}_j, \tilde{y}_j)  \right\|^2_{\mathrm{F}}  \\ 
  &\leq (t-t_c)n^2\eta^2 \frac{1}{K}\sum_{i=1}^K  \sum_{t'=t_c}^{t-1} \left\|   \nabla_{\mathbf{W}^{(i)}} \ell (\mathbf{W}^{(i)}(t'); \tilde{\bm{x}}_i, \tilde{y}_i)\right\|^2_{\mathrm{F}}\\ 
  & = (t-t_c)n^2\eta^2 \frac{1}{K}\sum_{i=1}^K  \sum_{t'=t_c}^{t-1}   \left\|   \mathbf{D}^{(i)}\bm{v}  \left(f(\mathbf{W}^{(i)}(t),\bm{v},\tilde{\bm{x}}_{i}) - \tilde{y}_{i} \right)  \tilde{\bm{x}}_{i} \right\|^2_{\mathrm{F}}\\
   & \leq (t-t_c)n^2\eta^2 \frac{m}{dK}\sum_{i=1}^K  \sum_{t'=t_c}^{t-1} \left(2\left\|     f(\mathbf{W}^{(i)}(t'),\bm{v},\tilde{\bm{x}}_i) - f(\mathbf{W} (t'),\bm{v},\tilde{\bm{x}}_i)    \right\|^2_{\mathrm{F}} +  2\left\|   f(\mathbf{W} (t'),\bm{v},\tilde{\bm{x}}_i)  \right\|^2_{\mathrm{F}}\right)\\
    & \leq 2(t-t_c)n^2\eta^2 \frac{m^2}{ d^2 }  \sum_{t'=t_c}^{t-1} \left( \frac{1}{K}\sum_{i=1}^K\left\|  \mathbf{W}^{(i)}(t')- \mathbf{W} (t')   \right\|^2_{\mathrm{F}} \right)+  4(t-t_c)n^2\eta^2 \frac{m}{ d}\sum_{t'=t_c}^{t-1} L(\mathbf{W} (t')).
\end{align*}
 
Let $a_t = \frac{1}{K}\sum_{i=1}^K   \left\|  \mathbf{W}^{(i)}(t)  -\mathbf{W}(t')   \right\|^2_{\mathrm{F}}  $ and $b_t =   L(\mathbf{W}(t)) $, so we have:
\begin{align*}
    a_t \leq \frac{2m^2}{ d^2 }(t-t_c)n^2 \eta^2 \sum_{t'=t_c}^{t-1} a_{t'} + \frac{4m}{ d} (t-t_c)n^2 \eta^2 \sum_{t'=t_c}^{t-1} b_{t'}. 
\end{align*}
Summing over $t$ from $t_c$ to $h$, where $t_c \leq h\leq t_c+\tau$:

\begin{align*}
    \sum_{t=t_c}^{h} a_t &\leq  \sum_{t=t_c}^{h}\frac{2m^2n^2}{ d^2 }(t-t_c) \eta^2 \sum_{t'=t_c}^{t-1} a_{t'} +  \sum_{t=t_c}^{h}\frac{4m n^2}{ d}  (t-t_c) \eta^2 \sum_{t'=t_c}^{t-1} b_{t'}\nonumber\\
    &\leq  \sum_{t=t_c}^{h}\frac{2m^2n^2}{ d^2 } \tau \eta^2 \sum_{t'=t_c}^{t-1} a_{t'} +  \sum_{t=t_c}^{h}\frac{4m n^2}{ d} \tau \eta^2 \sum_{t'=t_c}^{t-1} b_{t'}\nonumber\\
     &\leq  h \frac{2m^2n^2}{ d^2 } \tau \eta^2 \sum_{t'=t_c}^{h} a_{t'} +   h \frac{4m n^2}{ d} \tau \eta^2 \sum_{t'=t_c}^{h} b_{t'}\nonumber\\
     &\leq    \frac{2m^2n^2}{ d^2 } \tau^2 \eta^2 \sum_{t'=t_c}^{h} a_{t'} +    \frac{4m n^2}{ d}  \tau^2 \eta^2 \sum_{t'=t_c}^{h} b_{t'}\nonumber.
\end{align*}
Re-arranging the terms, and using the fact that $1- \frac{2m^2n^2}{ d^2 } \tau^2 \eta^2 \geq \frac{1}{2}$ yields:

\begin{align*}
    \sum_{t=t_c}^{h} a_t  \leq  \frac{8m n^2}{ d}   \tau^2 \eta^2 \sum_{t'=t_c}^{h} b_{t'}\nonumber.
\end{align*}
So, we can conclude that:
\begin{align*}
     a_t & \leq  \frac{2m^2n^2}{ d^2 }(t-t_c) \eta^2 \sum_{t'=t_c}^{t-1} a_{t'} +  \frac{4m n^2}{ d}  (t-t_c) \eta^2 \sum_{t'=t_c}^{t-1} b_{t'}\nonumber\\
     &\leq  \frac{2m^2n^2}{ d^2 }\tau \eta^2 \sum_{t'=t_c}^{t-1} a_{t'} + \frac{4m n^2}{ d}   \tau \eta^2 \sum_{t'=t_c}^{t-1} b_{t'}\nonumber\\
     &\leq \left(  \frac{16m^3n^4 \tau^3 \eta^4}{d^3}+ \frac{4m n^2}{ d} \tau \eta^2\right) \sum_{t'=t_c}^{t-1} b_{t'}\nonumber.
\end{align*}
\end{proof}
\end{lemma}

 \subsection{Proof of Theorem~\ref{theorem: local SGD}:}
 With the above lemmas in hand, we can finally proceed to the proof of Theorem~\ref{theorem: local SGD}.
 We prove Theorem~\ref{theorem: local SGD} by induction. Assume the following induction hypotheses hold for all $h \leq t$, with probability at least $1-O(n^{-1})$:
 \begin{align}
      &\textbf{(I)} \quad \left \| \mathbf{W}(h) -  \mathbf{W}(0)\right\| \leq \omega, \left \| \mathbf{W}^{(i)}(h) -  \mathbf{W}(0)\right\| \leq \omega, \forall i \in [K] \nonumber, \\
      &\textbf{(II)} \quad L(\mathbf{W}(h))   \le\left(1-  \Omega\left(\frac{\eta m \phi}{dn^2}\right)\right)^{h} nL( \mathbf{W}(0))\nonumber\\
&\quad \quad \quad \quad \quad \quad \quad \quad+  \exp\left[{  O  \left(  \frac{d^{1/2} n^{10}}{m^{1/2}\phi^{5/2}  }\right)   } \right] O\left(\frac{ m^{7/2}n^{11} \tau^3 \eta^3}{d^{3}  \phi^{3/2}}+  \frac{ m^{3/2}n^{9}\tau \eta   }{d^{1/2} \phi^{3/2} }\right)   L(\mathbf{W}(0))  \nonumber,
 \end{align}
 where $\omega = O\big(\phi^{3/2}n^{-9} \log^{-3/2}(m)\big)$. Then, we need to show that these two statements hold for $t+1$.
  \subsubsection{Proof of inductive hypothesis I}
  \paragraph{Step 1: Bounded virtual average iterates.}
  Now we prove the first hypothesis for $t+1$: $\left \| \mathbf{W}(t+1) -  \mathbf{W}(0)\right\| \leq \omega $. By the updating rule we know that:
   \begin{align}
      \left \| \mathbf{W}(t+1) -  \mathbf{W}(0)\right\| &\leq \eta \sum_{j=1}^t\left \|\frac{1}{K}\sum_{i=1}^K \mathbf{G}_i^{(j)}  \right\|_{\mathrm{F}} \nonumber\\
      &\leq \eta \sum_{j=1}^t\frac{1}{K}\sum_{i=1}^K\left \| n\nabla \ell  (\mathbf{W}^{(i)}(j);\tilde{\bm{x}}_{i_j},\tilde{y}_{i_j} )   - n\nabla \ell  (\mathbf{W}(j);\tilde{\bm{x}}_{i_j},\tilde{y}_{i_j} )  \right\|_{\mathrm{F}} \nonumber \\
      &\quad + \eta \sum_{j=1}^t\frac{1}{K}\sum_{i=1}^K\left \|n   \nabla \ell  (\mathbf{W}(j);\tilde{\bm{x}}_{i_j},\tilde{y}_{i_j} )  \right\|_{\mathrm{F}} \nonumber\\ 
      &\leq \eta \sum_{j=1}^t\sqrt{\frac{1}{K}\sum_{i=1}^K\left \| n\nabla \ell  (\mathbf{W}^{(i)}(j);\tilde{\bm{x}}_{i_j},\tilde{y}_{i_j} )   - n\nabla \ell  (\mathbf{W}(j);\tilde{\bm{x}}_{i_j},\tilde{y}_{i_j} )  \right\|^2_{\mathrm{F}}} \nonumber \\
      &\quad+ \eta \sum_{j=1}^t\sqrt{\frac{1}{K}\sum_{i=1}^K\left \|n   \nabla \ell  (\mathbf{W}(j);\tilde{\bm{x}}_{i_j},\tilde{y}_{i_j} )  \right\|^2_{\mathrm{F}}} \nonumber,
 \end{align} 
where $\tilde{\bm{x}}_{i_j},\tilde{y}_{i_j}$ denote the pair of randomly sampled data to compute stochastic gradient $\mathbf{G}_i^{(j)}$, and the last inequality is according to the concavity of $\sqrt{x}$ and Jensen's inequality.  Plugging in Lemma~\ref{lm: one point gradient gap} yields:
\begin{align}
      \left \| \mathbf{W}(t+1) -  \mathbf{W}(0)\right\| &\leq  n \eta\sum_{j=1}^t  \sqrt{ m L(\mathbf{W}(j))/d}\nonumber \\
      &\quad+   n\eta\sum_{j=1}^t   \sqrt{\frac{ 2m^2}{d^2K}\sum_{i=1}^K   \left\|   \mathbf{W}^{(i)}(j)    -     \mathbf{W}(j)   \right\|^2_{\mathrm{F}} +  \frac{2\omega^{2/3}m }{d} L(\mathbf{W}(j))}  \nonumber \\
       &\leq \underbrace{n \eta\sum_{j=1}^t  \sqrt{ mL(\mathbf{W}(j))/d}}_{\spadesuit} \nonumber \\
       &\quad+\underbrace{n\eta\sum_{j=1}^t   \sqrt{\frac{ 2m^2}{d^2 }\left(\left(  \frac{16m^3n^4 \tau^3 \eta^4}{d^3}+ \frac{4m n^2}{ d} \tau \eta^2\right) \sum_{t'=t_c}^{t-1}  L(\mathbf{W}(t')) \right) +  \frac{2\omega^{2/3}m }{d}  L(\mathbf{W}(j))}}_{\heartsuit}\nonumber, 
 \end{align} 
 
 where $t_c$ is the latest communication round at iteration $j$. Now we need to bound $\spadesuit$ and $\heartsuit$ separately. 
 
 We firstly bound $\spadesuit$ as follows. By plugging the convergence rate for $L(\mathbf{W}(j))$ we have:
 \begin{align*}
     \spadesuit &= n\eta\sum_{j=1}^t O\big(\sqrt{m  / d   }\big)\nonumber\\
     &\quad\sqrt{\left(1-  \Omega\left(\frac{\eta m \phi}{dn^2}\right)\right)^{j} nL( \mathbf{W}(0)) +  \exp\left[{  O  \left(  \frac{d^{1/2} n^{10}}{m^{1/2}\phi^{5/2}  }\right)   } \right] O\left(\frac{ m^{7/2}n^{11} \tau^3 \eta^3}{d^{3}  \phi^{3/2}}+  \frac{ m^{3/2}n^{9}\tau \eta   }{d^{1/2} \phi^{3/2} }\right)   L(\mathbf{W}(0)) }\nonumber\\
     &\stackrel{\text{\ding{192}}}{\leq} n\eta\sum_{j=1}^t O\big(\sqrt{m  /d}\big)\left(\sqrt{\left(1-  \Omega\left(\frac{\eta m \phi}{dn^2}\right)\right)^{j} nL( \mathbf{W}(0))}  \right)\nonumber\\
     &\quad+ n\eta\sum_{j=1}^t O\big(\sqrt{m  /d}\big)\left( \sqrt{\exp\left[{  O  \left(  \frac{d^{1/2} n^{10}}{m^{1/2}\phi^{5/2}  }\right)   } \right] O\left(\frac{ m^{7/2}n^{11} \tau^3 \eta^3}{d^{3}  \phi^{3/2}}+  \frac{ m^{3/2}n^{9}\tau \eta   }{d^{1/2} \phi^{3/2} }\right)   L(\mathbf{W}(0)) }\right)\nonumber \\
      &\stackrel{\text{\ding{193}}}{\leq} n^3  O\big(\sqrt{ nd  / m \phi}\big)      \nonumber\\
     &\quad+ n\eta t O\big(\sqrt{m  /d}\big)\left( \sqrt{\exp\left[{  O  \left(  \frac{d^{1/2} n^{10}}{m^{1/2}\phi^{5/2}  }\right)   } \right] O\left(\frac{ m^{7/2}n^{11} \tau^3 \eta^3}{d^{3}  \phi^{3/2}}+  \frac{ m^{3/2}n^{9}\tau \eta   }{d^{1/2} \phi^{3/2} }\right)   L(\mathbf{W}(0)) }\right)\nonumber, 
 \end{align*}
 where in \ding{192} we use triangle inequality to split square root, and in \ding{193} we use the fact $(1-a)^{1/2} \leq 1-\frac{a}{2}$, and $\sum_{j=1}^{\infty} \left(1-  \Omega\left(\frac{\eta m \phi}{2dn^2}\right)\right)^{j}  = O\left(\frac{2dn^2}{\eta m \phi}\right) $. Since we choose: $m \geq \frac{d n^{25} (\log m)^3}{\phi^4}$, $\eta = \frac{d n^2\log T}{m\phi T}$ and  hence
 $$T \geq  \frac{d  n^{22.5}   (\log T)^3 \tau(\log m)^{3/2 }}{  \phi^{11/2} }\exp\left[{  O  \left(  \frac{1 }{ n^{5/2}\phi^{1/2} (\log m)^{3/2}  }\right)   } \right]\geq \frac{d^{3/2} n^{35}   (\log T)^3 \tau(\log m)^{3 }}{m^{1/2} \phi^{15/2} }\exp\left[{  O  \left(  \frac{d^{1/2} n^{10}}{m^{1/2}\phi^{5/2}  }\right)   } \right],$$
 we conclude that $\spadesuit \leq \omega = O\big(\phi^{3/2}n^{-9} \log^{-3/2}(m)\big)$.
 
For $\heartsuit$:
 \begin{align*}
     \heartsuit &= n\eta\sum_{j=1}^t   \sqrt{\frac{ 2m^2}{d^2 }\left(\left(  \frac{16m^3n^4 \tau^3 \eta^4}{d^3}+ \frac{4m n^2}{ d} \tau \eta^2\right) \sum_{t'=t_c}^{t-1}  L(\mathbf{W}(t')) \right) +  \frac{2\omega^{2/3}m }{d}  L(\mathbf{W}(j))}\nonumber\\
    &\leq  n\eta   \sqrt{\frac{ 2m^2}{d^2 }\left(  \frac{16m^3n^4 \tau^3 \eta^4}{d^3}+ \frac{4m n^2}{ d} \tau \eta^2\right)   }  \underbrace{\sum_{j=1}^t\sqrt{   \sum_{t'=t_c}^{j-1} L(\mathbf{W}(t')) }}_{T_1} +  \underbrace{n\eta\sum_{j=1}^t\sqrt{\frac{2\omega^{2/3}m }{d} L(\mathbf{W}(j))}}_{T_2} \nonumber.
 \end{align*}
 $T_2$ is smaller than $\spadesuit$, so we know that $T_2 \leq \omega$. Now it only remains to bound $T_1$, so we again plug in the convergence rate of objective value: 
 \begin{align*}
     T_1 & \leq \sum_{j=1}^t  \sum_{t'=t_c}^{j-1}\sqrt{  \left(1-  \Omega\left(\frac{\eta m \phi}{dn^2}\right)\right)^{t'} nL( \mathbf{W}(0))}\\
     &\quad+ t\sqrt{ \exp\left[{  O  \left(  \frac{d^{1/2} n^{10}}{m^{1/2}\phi^{5/2}  }\right)   } \right] O\left(\frac{ m^{7/2}n^{11} \tau^3 \eta^3}{d^{3}  \phi^{3/2}}+  \frac{ m^{3/2}n^{9}\tau \eta   }{d^{1/2} \phi^{3/2} }\right)  L(\mathbf{W}(0)) }    \nonumber\\
         & \leq \tau\sum_{j=1}^t    \left(1-  \Omega\left(\frac{\eta m \phi}{2dn^2}\right)\right)^{t'} \sqrt{nL( \mathbf{W}(0))}\\
         &\quad+  t\sqrt{  \exp\left[{  O  \left(  \frac{d^{1/2} n^{10}}{m^{1/2}\phi^{5/2}  }\right)   } \right] O\left(\frac{ m^{7/2}n^{11} \tau^3 \eta^3}{d^{3}  \phi^{3/2}}+  \frac{ m^{3/2}n^{9}\tau \eta   }{d^{1/2} \phi^{3/2} }\right)  L(\mathbf{W}(0)) } \nonumber\\
           & \leq \tau O\left(\frac{2dn^2}{\eta m \phi}\right)  \sqrt{nL( \mathbf{W}(0))}    \nonumber\\
            &\quad+  t\sqrt{  \exp\left[{  O  \left(  \frac{d^{1/2} n^{10}}{m^{1/2}\phi^{5/2}  }\right)   } \right] O\left(\frac{ m^{7/2}n^{11} \tau^3 \eta^3}{d^{3}  \phi^{3/2}}+  \frac{ m^{3/2}n^{9}\tau \eta   }{d^{1/2} \phi^{3/2} }\right)   L(\mathbf{W}(0)) } \nonumber.
 \end{align*}

So we can conclude that:
\begin{align*} 
 \heartsuit &  \leq   \eta^2   \sqrt{\frac{ 2m^3n^3\tau }{d^3 }   } \left( O\left(\frac{ \tau d n^{2.5}}{\eta m \phi}\right)   +  t\sqrt{ \exp\left[{  O  \left(  \frac{d^{1/2} n^{10}}{m^{1/2}\phi^{5/2}  }\right)   } \right] O\left(\frac{ m^{7/2}n^{11} \tau^3 \eta^3}{d^{3}  \phi^{3/2}}+  \frac{ m^{3/2}n^{9}\tau \eta   }{d^{1/2} \phi^{3/2} }\right)  }  \right)  + O(\omega) \nonumber\\
  &  \leq    O\left(\frac{\tau^{3/2} m^{1/2}  n^{4}\eta}{d^{1/2}  \phi}\right)   + \eta^2  t\sqrt{ \exp\left[{  O  \left(  \frac{d^{1/2} n^{10}}{m^{1/2}\phi^{5/2}  }\right)   } \right] O\left(\frac{ m^{7/2}n^{11} \tau^3 \eta^3}{d^{3}  \phi^{3/2}}+  \frac{ m^{3/2}n^{9}\tau \eta   }{d^{1/2} \phi^{3/2} }\right) }    + O(\omega) \nonumber.
\end{align*}
According to our choice of $\eta$, $T$ and $m$:
$$T \geq  \tau^{3/2} n^{5/2}\phi^{1/2}\log T   \geq \frac{\tau^{3/2}d^{1/2}n^{15}\log T (\log m)^{3/2}}{m^{1/2}\phi^{7/2}}$$

we conclude that $\heartsuit\leq \omega$.
\paragraph{Step 2: Bounded local iterates.} Now we verify the second statement in hypothesis (\textbf{I}), the boundedness of local iterates. For any $i \in [K]$, we have:
 \begin{align}
      \left \| \mathbf{W}^{(i)}(t+1) -  \mathbf{W}(0)\right\| & \leq \left \| \mathbf{W}^{(i)}(t+1) -  \mathbf{W}(t+1) \right\| + \left \| \mathbf{W}(t+1) -  \mathbf{W}(0)\right\|\nonumber. 
 \end{align}
 Since we know that $\left \| \mathbf{W}(t+1) -  \mathbf{W}(0)\right\| \leq O(\omega)$ from step a, then it remains to verify $\left\| \mathbf{W}^{(i)}(t+1) -  \mathbf{W}(t+1) \right\|\leq O(\omega)$. According to Lemma~\ref{lemma: weight gap SGD non expectation}:
 \begin{align*}
    \left\| \mathbf{W}^{(i)}(t+1) -  \mathbf{W}(t+1) \right\| &\leq K \cdot \frac{1}{K}\sum_{i=1}^K \sqrt{\left\| \mathbf{W}^{(i)}(t) -  \mathbf{W}(t) \right\|^2 } \leq K \cdot  \sqrt{\frac{1}{K}\sum_{i=1}^K\left\| \mathbf{W}^{(i)}(t) -  \mathbf{W}(t) \right\|^2_{\mathrm{F}} } \\
    &\leq K\sqrt{\left(  \frac{16m^3n^4 \tau^3 \eta^4}{d^3}+ \frac{4m n^2}{ d} \tau \eta^2\right) \sum_{t'=t_c}^{t-1}  L(\mathbf{W}(t'))}.
 \end{align*}
 We plug in the bound of loss from hypothesis (\textbf{II}), and obtain:
  \begin{align*}
    &\left\| \mathbf{W}^{(i)}(t+1) -  \mathbf{W}(t+1) \right\| \\  
    &\leq K\sqrt{\left(\frac{16m^3n^4 \tau^3 \eta^4}{d^3}+ \frac{4m n^2}{ d} \tau \eta^2\right)}\\
    &\quad\sqrt{\sum_{t'=t_c}^{t-1}\left[ \left(1-  \Omega\left(\frac{\eta m \phi}{dn^2}\right)\right)^{t'} L( \mathbf{W}(0))  +  \exp\left[{  O  \left(  \frac{d^{1/2} n^{10}}{m^{1/2}\phi^{5/2}  }\right)   } \right] O\left(\frac{ m^{7/2}n^{11} \tau^3 \eta^3}{d^{3}  \phi^{3/2}}+  \frac{ m^{3/2}n^{9}\tau \eta   }{d^{1/2} \phi^{3/2} }\right)   L(\mathbf{W}(0)) \right]}\\
      &\leq K\sqrt{\left(\frac{16m^3n^4 \tau^3 \eta^4}{d^3}+ \frac{4m n^2}{ d} \tau \eta^2\right)}\\
    & \quad\sqrt{\tau \left[  L( \mathbf{W}(0))  + \exp\left[{  O  \left(  \frac{d^{1/2} n^{10}}{m^{1/2}\phi^{5/2}  }\right)   } \right] O\left(\frac{ m^{7/2}n^{11} \tau^3 \eta^3}{d^{3}  \phi^{3/2}}+  \frac{ m^{3/2}n^{9}\tau \eta   }{d^{1/2} \phi^{3/2} }\right)   L(\mathbf{W}(0)) \right]}.
 \end{align*}
 Since we choose 
 \begin{align*}
     T \geq \frac{K \tau  \log T}{n^{1/2}\phi^{1/2}} \geq \frac{K \tau d^{1/2} n^{12} \log T (\log m)^{3/2}}{m^{1/2} \phi^{5/2} },
 \end{align*}
 we can conclude that $\left\| \mathbf{W}^{(i)}(t+1) -  \mathbf{W}(t+1) \right\| \leq O(\omega)$.

\subsubsection{Proof of inductive hypothesis II}
\paragraph{Step 1: One iteration analysis from semi-smoothness.}
 Now we switch to prove the hypothesis \textbf{II}. According to semi-smoothness and updating rule we have:
\begin{align*} 
L(\mathbf{W}(t+1))&\le L( \mathbf{W}(t)) + \left\langle \nabla L( \mathbf{W}(t)),   \mathbf{W}(t+1)-  \mathbf{W}(t)\right \rangle \notag\\
&\quad  + C'\sqrt{nL(\mathbf{W}(t))}\cdot\frac{\omega^{1/3}\sqrt{m\log(m)}}{\sqrt{d}}\cdot \|\mathbf{W}(t+1)-  \mathbf{W}(t)\| + \frac{C''nm}{d}\|\mathbf{W}(t+1)- \mathbf{W}(t)\|^2\\
&\le L( \mathbf{W}(t)) - \left\langle \nabla L( \mathbf{W}(t)),    \eta \frac{1}{K}\sum_{i=1}^K G^{(t)}_i\right \rangle  +\eta C'\sqrt{nL(\mathbf{W}(t))}\cdot\frac{\omega^{1/3}\sqrt{m\log(m)}}{\sqrt{d}}\cdot \left\|\frac{1}{K}\sum_{i=1}^K  G^{(t)}_i\right \|\\
&\quad+ \eta^2\frac{C''nm}{d}\left\|\frac{1}{K}\sum_{i=1}^K G^{(t)}_i\right\|^2 .
\end{align*}
We let $S_t$ be the set of sampled data to compute stochastic gradient, at iteration $t$. Taking expectation over $S_t$ on both sides:
\begin{align*} 
&\mathbb{E}_{S_t}\left[L(\mathbf{W}(t+1))\right]\\
& \stackrel{\text{\ding{192}}}{\leq}  L( \mathbf{W}(t))  -  \frac{\eta}{2} \left\| \nabla L( \mathbf{W}(t)) \right\|^2_{\mathrm{F}}  -\frac{\eta}{2} \left\| \frac{1}{K}\sum_{i=1}^K \nabla  L_i(\mathbf{W}^{(i)}(t)) \right \|^2_{\mathrm{F}}  +\frac{\eta}{2}  \left\| \nabla L( \mathbf{W}(t))-\frac{1}{K}\sum_{i=1}^K \nabla  L_i(\mathbf{W}^{(i)}(t)) \right \|^2_{\mathrm{F}}   \\
&\quad+\eta C'\sqrt{nL(\mathbf{W}(t))}  \cdot\frac{\omega^{1/3}\sqrt{m\log(m)}}{2\sqrt{d}}  \mathbb{E}_{S_t}\left[\left\|\frac{1}{K}\sum_{i=1}^K G^{(t)}_i \right \|\right]  +  \eta^2 \frac{C''nm}{d}\mathbb{E}_{S_t}\left[\left\| \frac{1}{K}\sum_{i=1}^K G^{(t)}_i\right\|^2\right]\\
&\le  L( \mathbf{W}(t))  -  \frac{\eta}{2} \left\| \nabla L( \mathbf{W}(t)) \right\|^2_{\mathrm{F}}  +\frac{\eta}{2} \frac{1}{K}\sum_{i=1}^K  \left\| \nabla L_i( \mathbf{W}(t))-\nabla  L_i(\mathbf{W}^{(i)}(t)) \right \|^2_{\mathrm{F}}  \\
& \quad   +\eta C' \sqrt{nL(\mathbf{W}(t))}  \cdot\frac{\omega^{1/3}\sqrt{m\log(m)}}{2\sqrt{d}} \sqrt{\mathbb{E}_{S_t}\left[\left\|\frac{1}{K}\sum_{i=1}^K G^{(t)}_i \right \|^2\right]}+  \eta^2 \frac{C''nm}{d}\mathbb{E}_{S_t}\left[\left\| \frac{1}{K}\sum_{i=1}^K G^{(t)}_i\right\|^2\right] ,
\end{align*} 
where in \ding{192} we use the identity $\langle \bm{v},\bm{b} \rangle =  \frac{1}{2}\|\bm{v} \|^2+\frac{1}{2}\| \bm{b}\|^2 - \frac{1}{2}\|\bm{v}-\bm{b}\|^2$. 
We plug in Lemma~\ref{lm: gradient gap} and \ref{lemma: bounded variance}:
\begin{align*} 
&\mathbb{E}_{S_t}\left[L(\mathbf{W}(t+1))\right]\\ 
&\le  L( \mathbf{W}(t))  -  \frac{\eta}{2} \left\| \nabla L( \mathbf{W}(t)) \right\|^2_{\mathrm{F}}  +\frac{\eta}{2} \left(\frac{2 m^2n^2}{d^2}\frac{1}{K}\sum_{i=1}^K   \left\|   \mathbf{W}^{(i)}(t)    -     \mathbf{W}(t)   \right\|^2_{\mathrm{F}}  +  \frac{C\omega^{2/3}  mn\log(m)}{d} L(\mathbf{W}(t)) \right)\\
& \quad   +\eta C' \sqrt{nL(\mathbf{W}(t))}  \cdot\frac{\omega^{1/3}\sqrt{m\log(m)}}{2\sqrt{d}} \sqrt{\frac{2m^2n^2}{d^2}\frac{1}{ K^2}\sum_{i=1}^K\left \|  \mathbf{W}^{(i)}(t)  -  \mathbf{W}(t) \right\|^2_{\mathrm{F}}  +   \frac{2mn}{dK}L(\mathbf{W} (t) )}\\
&+  \eta^2 \frac{C''nm}{d} \left[\frac{2m^2n^2}{d^2}\frac{1}{ K^2}\sum_{i=1}^K\left \|  \mathbf{W}^{(i)}(t)  -  \mathbf{W}(t) \right\|^2_{\mathrm{F}}  +   \frac{2mn}{dK}L(\mathbf{W} (t) )\right]\notag\\
&\le  L( \mathbf{W}(t))  -  \frac{\eta}{2} \left\| \nabla L( \mathbf{W}(t)) \right\|^2_{\mathrm{F}}  + \left(  \frac{C\omega^{2/3}  mn\log(m)\eta}{2d} +  \eta^2 \frac{C''nm}{d} \frac{2mn}{dK} \right)L(\mathbf{W}(t))\\
& \quad   +\eta C' \sqrt{nL(\mathbf{W}(t))}  \cdot\frac{\omega^{1/3}\sqrt{m\log(m)}}{2\sqrt{d}} \sqrt{\frac{2m^2n^2}{d^2}\frac{1}{ K^2}\sum_{i=1}^K\left \|  \mathbf{W}^{(i)}(t)  -  \mathbf{W}(t) \right\|^2_{\mathrm{F}}  +   \frac{2mn}{dK}L(\mathbf{W} (t) )}\\
&\quad +   \left(\frac{C''2m^3n^3\eta^2}{d^3 K}+\frac{  m^2n^2\eta}{d^2} \right)\frac{1}{K}\sum_{i=1}^K   \left\|   \mathbf{W}^{(i)}(t)    -     \mathbf{W}(t)   \right\|^2_{\mathrm{F}} \notag.
\end{align*}  
Applying the triangle inequality to split square root yields:
\begin{align*} 
\mathbb{E}_{S_t}\left[L(\mathbf{W}(t+1))\right] &\le  L( \mathbf{W}(t))  -  \frac{\eta}{2} \left\| \nabla L( \mathbf{W}(t)) \right\|^2_{\mathrm{F}}  + \left(  \frac{C\omega^{2/3}  mn\log(m)\eta}{2d} +  \eta^2 \frac{C''nm}{d} \frac{2mn}{dK} \right)L(\mathbf{W}(t))\\
& \quad   +\eta C' \sqrt{nL(\mathbf{W}(t))}  \cdot\frac{\omega^{1/3}\sqrt{m\log(m)}}{2\sqrt{d}} \left(\sqrt{\frac{2m^2n^2}{d^2}\frac{1}{ K^2}\sum_{i=1}^K\left \|  \mathbf{W}^{(i)}(t)  -  \mathbf{W}(t) \right\|^2_{\mathrm{F}} } +\sqrt{   \frac{2mn}{dK}L(\mathbf{W} (t) )}\right)\\
&\quad+   \left(\frac{C''2m^3n^3\eta^2}{d^3 K}+\frac{  m^2n^2\eta}{d^2} \right)\frac{1}{K}\sum_{i=1}^K   \left\|   \mathbf{W}^{(i)}(t)    -     \mathbf{W}(t)   \right\|^2_{\mathrm{F}} \\
&\le  L( \mathbf{W}(t))  -  \frac{\eta}{2} \left\| \nabla L( \mathbf{W}(t)) \right\|^2_{\mathrm{F}}  + \left(  \frac{C\omega^{2/3}  mn\log(m)\eta}{2d} +     \frac{C'' m^2n^2\eta^2}{d^2K} + \frac{\omega^{1/3}mn\sqrt{\log (m)}\eta}{d\sqrt{K}} \right)L(\mathbf{W}(t))\\ 
&\quad+   \left(\frac{C''2m^3n^3\eta^2}{d^3 K}+\frac{  m^2n^2\eta}{d^2}  +   \frac{\eta C'\omega^{1/3}m^{5/2}n^{5/2}\sqrt{ \log(m)}}{4d^{5/2}K}  \right)\frac{1}{K}\sum_{i=1}^K   \left\|   \mathbf{W}^{(i)}(t)    -     \mathbf{W}(t)   \right\|^2_{\mathrm{F}}  .
\end{align*}

We further take expectation over $\{S_1,...,S_t\}$, choose $\omega = \frac{\phi^{3/2}}{C_\omega n^9(\log(m))^{3/2}}$ where $C$ is some large constant, and plug in Lemma~\ref{lemma:grad bounds} and Lemma~\ref{lemma: weight gap SGD non expectation}:
\begin{align*} 
\mathbb{E}[L(\mathbf{W}(t+1))]  &\le \left(1-  \Omega\left(\frac{\eta m \phi}{dn^2}\right)\right) \mathbb{E}[L( \mathbf{W}(t))]  \nonumber\\
& \quad+O \left(\frac{  m^2n^2\eta}{d^2}  +\frac{\eta C'\omega^{1/3}m^{5/2}n^{5/2}\sqrt{ \log(m)}}{4d^{5/2}K}  \right)\left(  \frac{16m^3n^4 \tau^3 \eta^4}{d^3}+ \frac{4m n^2\tau \eta^2}{ d} \right) \sum_{t'=t_c}^{t-1}  L(\mathbf{W}(t'))\nonumber\\
&  \le \left(1-  \Omega\left(\frac{\eta m \phi}{dn^2}\right)\right) \mathbb{E}[L( \mathbf{W}(t))]  \nonumber\\
&\quad + O\left(  \frac{ m^{11/2}n^{7/2} \tau^3 \eta^5\phi^{1/2}}{d^{11/2}K}+  \frac{ m^{7/2}n^{3/2}\tau \eta^3 \phi^{1/2}}{d^{5/2}K} + \frac{m^5n^6\tau^3\eta^5}{d^5}+\frac{m^3n^4\tau \eta^3}{d^3}\right)\sum_{t'=t_c}^{t-1} \mathbb{E}\left[L(\mathbf{W}(t'))\right]\nonumber\\
&\le\left(1-  \Omega\left(\frac{\eta m \phi}{dn^2}\right)\right) \mathbb{E}[L( \mathbf{W}(t))]  \\
&\quad+ O\left(\frac{ m^{11/2}n^{6} \tau^3 \eta^5\phi^{1/2}}{d^{5} }+  \frac{ m^{7/2}n^{4}\tau \eta^3 \phi^{1/2}}{d^{5/2} }\right) \sum_{t'=t_c}^{t-1} \mathbb{E}[L(\mathbf{W}(t'))] .
\end{align*}
  \paragraph{Step 2: Reducing cumulative loss to loss at communication round.}
 We firstly need to bound $\sum_{t'=t_c}^{t-1} L(\mathbf{W}(t')) $, which is the cumulative losses over between two communication rounds. We handle it by summing $t$ from $t_c$ to $h$, where $t_c\leq h \leq t_c+\tau$:
  
\begin{align*} 
\sum_{t=t_c}^h \mathbb{E}[L(\mathbf{W}(t+1))]  
&\le\left(1-  \Omega\left(\frac{\eta m \phi}{dn^2}\right)\right)\sum_{t=t_c}^h \mathbb{E}[L( \mathbf{W}(t))]  \\
&\quad + O\left(\frac{ m^{11/2}n^{6} \tau^3 \eta^5\phi^{1/2}}{d^{5} }+  \frac{ m^{7/2}n^{4}\tau \eta^3 \phi^{1/2}}{d^{5/2} }\right)\sum_{t=t_c}^h \sum_{t'=t_c}^{t-1} \mathbb{E}[L(\mathbf{W}(t'))] .
\end{align*}  
The LHS can be equivalently written as:  
  \begin{align*} 
\sum_{t=t_c+1}^{h+1} L(\mathbf{W}(t))  
&\le\left(1-  \Omega\left(\frac{\eta m \phi}{dn^2}\right)\right)\sum_{t=t_c}^h L( \mathbf{W}(t)) \\
&\quad +  O\left(\frac{ m^{11/2}n^{6} \tau^3 \eta^5\phi^{1/2}}{d^{5} }+  \frac{ m^{7/2}n^{4}\tau \eta^3 \phi^{1/2}}{d^{5/2} }\right)\sum_{t=t_c}^h \sum_{t'=t_c}^{t-1} L(\mathbf{W}(t')) \nonumber\\
&\le\left(1-  \Omega\left(\frac{\eta m \phi}{dn^2}\right)\right)\sum_{t=t_c+1}^{h+1} L( \mathbf{W}(t)) + \left(1-  \Omega\left(\frac{\eta m \phi}{dn^2}\right)\right)  L( \mathbf{W}(t_c))\nonumber\\
&\quad +O\left(\frac{ m^{11/2}n^{6} \tau^3 \eta^5\phi^{1/2}}{d^{5} }+  \frac{ m^{7/2}n^{4}\tau \eta^3 \phi^{1/2}}{d^{5/2} }\right) h\sum_{t'=t_c}^{h} L(\mathbf{W}(t')) \nonumber.
\end{align*}

Re-arranging the terms yields:
 \begin{align*} 
\Omega\left(\frac{\eta m \phi}{dn^2}\right)\sum_{t=t_c+1}^{h+1} L(\mathbf{W}(t))  
&\le \left(1-  \Omega\left(\frac{\eta m \phi}{dn^2}\right)\right)L(\mathbf{W}(t_c))\nonumber\\
& \quad+ O\left(\frac{ m^{11/2}n^{6} \tau^3 \eta^5\phi^{1/2}}{d^{5} }+  \frac{ m^{7/2}n^{4}\tau \eta^3 \phi^{1/2}}{d^{5/2} }\right)h\sum_{t'=t_c}^{h} L(\mathbf{W}(t')) \nonumber.
\end{align*}
Dividing both sides with $\Omega\left(\frac{\eta m \phi}{dn^2}\right)$ gives:

 \begin{align*} 
 \sum_{t=t_c+1}^{h+1} L(\mathbf{W}(t)) 
&\le O\left(\frac{dn^2}{\eta m \phi}\right)L(\mathbf{W}(t_c))+  O\left(\frac{ m^{9/2}n^{8} \tau^3 \eta^4}{d^{4}\phi^{1/2} }+  \frac{ m^{5/2}n^{6}\tau \eta^2 }{d^{3/2}\phi^{1/2} }\right) h\sum_{t'=t_c}^{h} L(\mathbf{W}(t')) \nonumber.
\end{align*}
We further re-write the LHS of the above inequality:
 \begin{align*} 
 \sum_{t=t_c}^{h} L(\mathbf{W}(t)) + L(\mathbf{W}(h+1)) -L(\mathbf{W}(t_c))
&\le O\left(\frac{dn^2}{\eta m \phi}\right)L(\mathbf{W}(t_c))\nonumber\\
&\quad+ O\left(\frac{ m^{9/2}n^{8} \tau^3 \eta^4}{d^{4}\phi^{1/2} }+  \frac{ m^{5/2}n^{6}\tau \eta^2 }{d^{3/2}\phi^{1/2} }\right)\tau\sum_{t'=t_c}^{h} L(\mathbf{W}(t')) \nonumber.
\end{align*}

By re-arranging terms we can conclude that:
 \begin{align*} 
 \sum_{t=t_c}^{h} L(\mathbf{W}(t))  
&\leq \frac{O\left(\frac{dn^2}{\eta m \phi}\right)}{ \Omega\left( 1- \left(\frac{ m^{9/2}n^{8} \tau^3 \eta^4}{d^{4}\phi^{1/2} }+  \frac{ m^{5/2}n^{6}\tau \eta^2 }{d^{3/2}\phi^{1/2} }\right)\tau \right)} L(\mathbf{W}(t_c)).  
\end{align*}
According to our choice of $n$, $\tau$ and $\eta$, $\frac{1}{ \Omega\left( 1- \left(\frac{ m^{9/2}n^{8} \tau^3 \eta^4}{d^{4}\phi^{1/2} }+  \frac{ m^{5/2}n^{6}\tau \eta^2 }{d^{3/2}\phi^{1/2} }\right)\tau \right)} = O(1)$. So we conclude:
\begin{align} 
L(\mathbf{W}(t+1))   
&\le \left(1-  \Omega\left(\frac{\eta m \phi}{dn^2}\right)\right)L( \mathbf{W}(t))\nonumber \\
&\quad+  O\left(\frac{ m^{11/2}n^{6} \tau^3 \eta^5\phi^{1/2}}{d^{5} }+  \frac{ m^{7/2}n^{4}\tau \eta^3 \phi^{1/2}}{d^{5/2} }\right)O\left(\frac{dn ^2}{\eta m \phi}\right) L(\mathbf{W}(t_c))   \nonumber  \\
&\le \left(1-  \Omega\left(\frac{\eta m \phi}{dn^2}\right)\right)L( \mathbf{W}(t))  +  O\left(\frac{ m^{9/2}n^{8} \tau^3 \eta^4}{d^{4}  \phi^{1/2}}+  \frac{ m^{5/2}n^{6}\tau \eta^2  }{d^{3/2} \phi^{1/2} }\right) L(\mathbf{W}(t_c))  \label{eq: proof_SGD_1},
\end{align}

where $t_c$ is the latest communication round before $t$, also the $c$-th communication round. 

\paragraph{Step 3: Bounded loss at communication rounds.}
It remains to bound $L(\mathbf{W}(t_c))$, the objective value at communication round. We handle it by summing above inequality over $t $ from $t_{c+1}$ to $t_c$: 
\begin{align*} 
 L(\mathbf{W}(t_{c+1}))   
&\le  \left(1-  \Omega\left(\frac{\eta m \phi}{dn^2 }\right)\right)^\tau L( \mathbf{W}(t_{c}))\nonumber\\
& \quad+    \sum_{j=1}^\tau \left(1-  \Omega\left(\frac{\eta m \phi}{dn^2 }\right)\right)^j O\left(\frac{ m^{9/2}n^{8} \tau^3 \eta^4}{d^{4}  \phi^{1/2}}+  \frac{ m^{5/2}n^{6}\tau \eta^2  }{d^{3/2} \phi^{1/2} }\right) L(\mathbf{W}(t_c))  \nonumber \\
&\le  \left[\left(1-  \Omega\left(\frac{\eta m \phi}{dn^2 }\right)\right)^\tau   +   O\left(\frac{ m^{9/2}n^{8} \tau^3 \eta^4}{d^{4}  \phi^{1/2}}+  \frac{ m^{5/2}n^{6}\tau \eta^2  }{d^{3/2} \phi^{1/2} }\right) \tau\right] L(\mathbf{W}(t_c))  \nonumber \\
&\le  \left[\left(1-  \Omega\left(\frac{\eta m \phi}{dn^2 }\right)\right)^\tau   +     O\left(\frac{ m^{9/2}n^{8} \tau^4 \eta^4}{d^{4}  \phi^{1/2}}+  \frac{ m^{5/2}n^{6}\tau^2 \eta^2  }{d^{3/2} \phi^{1/2} }\right)\right]^c L(\mathbf{W}(0))  \nonumber.
\end{align*}
Plugging in $\eta = \frac{d n^2\log T}{m\phi T}$, and letting $T = S\tau$ we have:
\begin{align*} 
 L(\mathbf{W}(t_{c+1}))   
&\le  \left[O\left(\frac{1}{T}\right)^{\frac{1}{S}}   +   O\left(\frac{ m^{9/2}n^{8} \tau^4 \eta^4}{d^{4}  \phi^{1/2}}+  \frac{ m^{5/2}n^{6}\tau^2 \eta^2  }{d^{3/2} \phi^{1/2} }\right) \right]^c L(\mathbf{W}(0))  \nonumber  \\ 
&=  \left(O\left(\frac{1}{T}\right)^{\frac{1}{S}} \right)^c\left[1   +    O\left(\frac{ m^{1/2}n^{16} \tau^4 (\log (T))^4}{  \phi^{9/2} T^{4-1/S}}+  \frac{d^{1/2} m^{1/2}n^{10}\tau^2 (\log (T))^2  }{ \phi^{5/2} T^{2-1/S} }\right)  \right]^c L(\mathbf{W}(0))  \nonumber \\
&\stackrel{\text{\ding{192}}}{\leq}  \left[1   +    O  \left(  \frac{ d^{1/2} n^{10}   }{m^{1/2}\phi^{5/2}    S}\right)    \right]^S L(\mathbf{W}(0))  \nonumber \\
&\leq \left[1   +   O  \left(  \frac{ d^{1/2} n^{10}   }{m^{1/2}\phi^{5/2}    S}\right)    \right]^{ O  \left(  \frac{\phi^{5/2} m^{1/2}  S}{  n^{10}    d^{1/2}    }\right)  O  \left(  \frac{  n^{10}    d^{1/2}     }{m^{1/2}\phi^{5/2}  }\right)   } L(\mathbf{W}(0))  \nonumber \\
&\leq    \exp\left[{  O  \left(  \frac{d^{1/2} n^{10}}{m^{1/2}\phi^{5/2}  }\right)   } \right]L(\mathbf{W}(0))  \nonumber,
\end{align*}
where in $\text{\ding{192}}$ we use our choice of $\tau$ and $T$ such that $\frac{\tau^2 (\log T)^2}{T^{2-\frac{1}{S}}} \leq \frac{1}{Sm}$.

\paragraph{Step 4: Sub-linear convergence of global loss.}
Now we can finally bound $L(\mathbf{W}(t+1)) $ by unrolling the recursion in (\ref{eq: proof_SGD_1}): 
\begin{align*} 
\mathbb{E}[L(\mathbf{W}(t+1))]   
&\le \left(1-  \Omega\left(\frac{\eta m \phi}{dn^2}\right)\right)L( \mathbf{W}(t)) \\
&\quad +  \exp\left[{  O  \left(  \frac{d^{1/2} n^{10}}{m^{1/2}\phi^{5/2}  }\right)   } \right]O\left(\frac{ m^{9/2}n^{8} \tau^3 \eta^4}{d^{4}  \phi^{1/2}}+  \frac{ m^{5/2}n^{6}\tau \eta^2  }{d^{3/2} \phi^{1/2} }\right)  \sum_{j=1}^t \left(1-  \Omega\left(\frac{\eta m \phi}{dn^2}\right)\right)^j  \mathbb{E}[L(\mathbf{W}(0))]  \nonumber\\
 & \le\left(1-  \Omega\left(\frac{\eta m \phi}{dn^2}\right)\right)^{t+1} L( \mathbf{W}(0))\nonumber\\
&\quad+  \exp\left[{  O  \left(  \frac{d^{1/2} n^{10}}{m^{1/2}\phi^{5/2}  }\right)   } \right]O\left(\frac{ m^{9/2}n^{8} \tau^3 \eta^4}{d^{4}  \phi^{1/2}}+  \frac{ m^{5/2}n^{6}\tau \eta^2  }{d^{3/2} \phi^{1/2} }\right) \sum_{j=1}^t  \left(1-  \Omega\left(\frac{\eta m \phi}{dn^2}\right)\right)^j     L(\mathbf{W}(0))  \nonumber\\
 & \le\left(1-  \Omega\left(\frac{\eta m \phi}{dn^2}\right)\right)^{t+1} L( \mathbf{W}(0))\nonumber\\
&\quad+  \exp\left[{  O  \left(  \frac{d^{1/2} n^{10}}{m^{1/2}\phi^{5/2}  }\right)   } \right]O\left(\frac{ m^{9/2}n^{8} \tau^3 \eta^4}{d^{4}  \phi^{1/2}}+  \frac{ m^{5/2}n^{6}\tau \eta^2  }{d^{3/2} \phi^{1/2} }\right) O\left(\frac{dn^2}{\eta m \phi}\right)    L(\mathbf{W}(0))  \nonumber\\ 
 & \le\left(1-  \Omega\left(\frac{\eta m \phi}{dn^2}\right)\right)^{t+1} L( \mathbf{W}(0))\nonumber\\
&\quad+  \exp\left[{  O  \left(  \frac{d^{1/2} n^{10}}{m^{1/2}\phi^{5/2}  }\right)   } \right] O\left(\frac{ m^{7/2}n^{10} \tau^3 \eta^3}{d^{3}  \phi^{3/2}}+  \frac{ m^{3/2}n^{8}\tau \eta   }{d^{1/2} \phi^{3/2} }\right)  L(\mathbf{W}(0))  \nonumber.
\end{align*}
Finally, according to Markov's inequality, with probability at least $1-O(n^{-1})$, we have:
\begin{align*} 
L(\mathbf{W}(t+1))  
 & \le\left(1-  \Omega\left(\frac{\eta m \phi}{dn^2}\right)\right)^{t+1} nL( \mathbf{W}(0))\nonumber\\
& \quad+  \exp\left[{  O  \left(  \frac{d^{1/2} n^{10}}{m^{1/2}\phi^{5/2}  }\right)   } \right] O\left(\frac{ m^{7/2}n^{11} \tau^3 \eta^3}{d^{3}  \phi^{3/2}}+  \frac{ m^{3/2}n^{9}\tau \eta   }{d^{1/2} \phi^{3/2} }\right)   L(\mathbf{W}(0))  \nonumber.
\end{align*}
\qed
\vspace{-0.25cm}
